# Supplementary material for: On prior smoothing with discrete spatial data in the context of disease mapping
Source: arXiv:2503.16151 source file (2025-07-29)

# MSS

$\mu = 0.002$

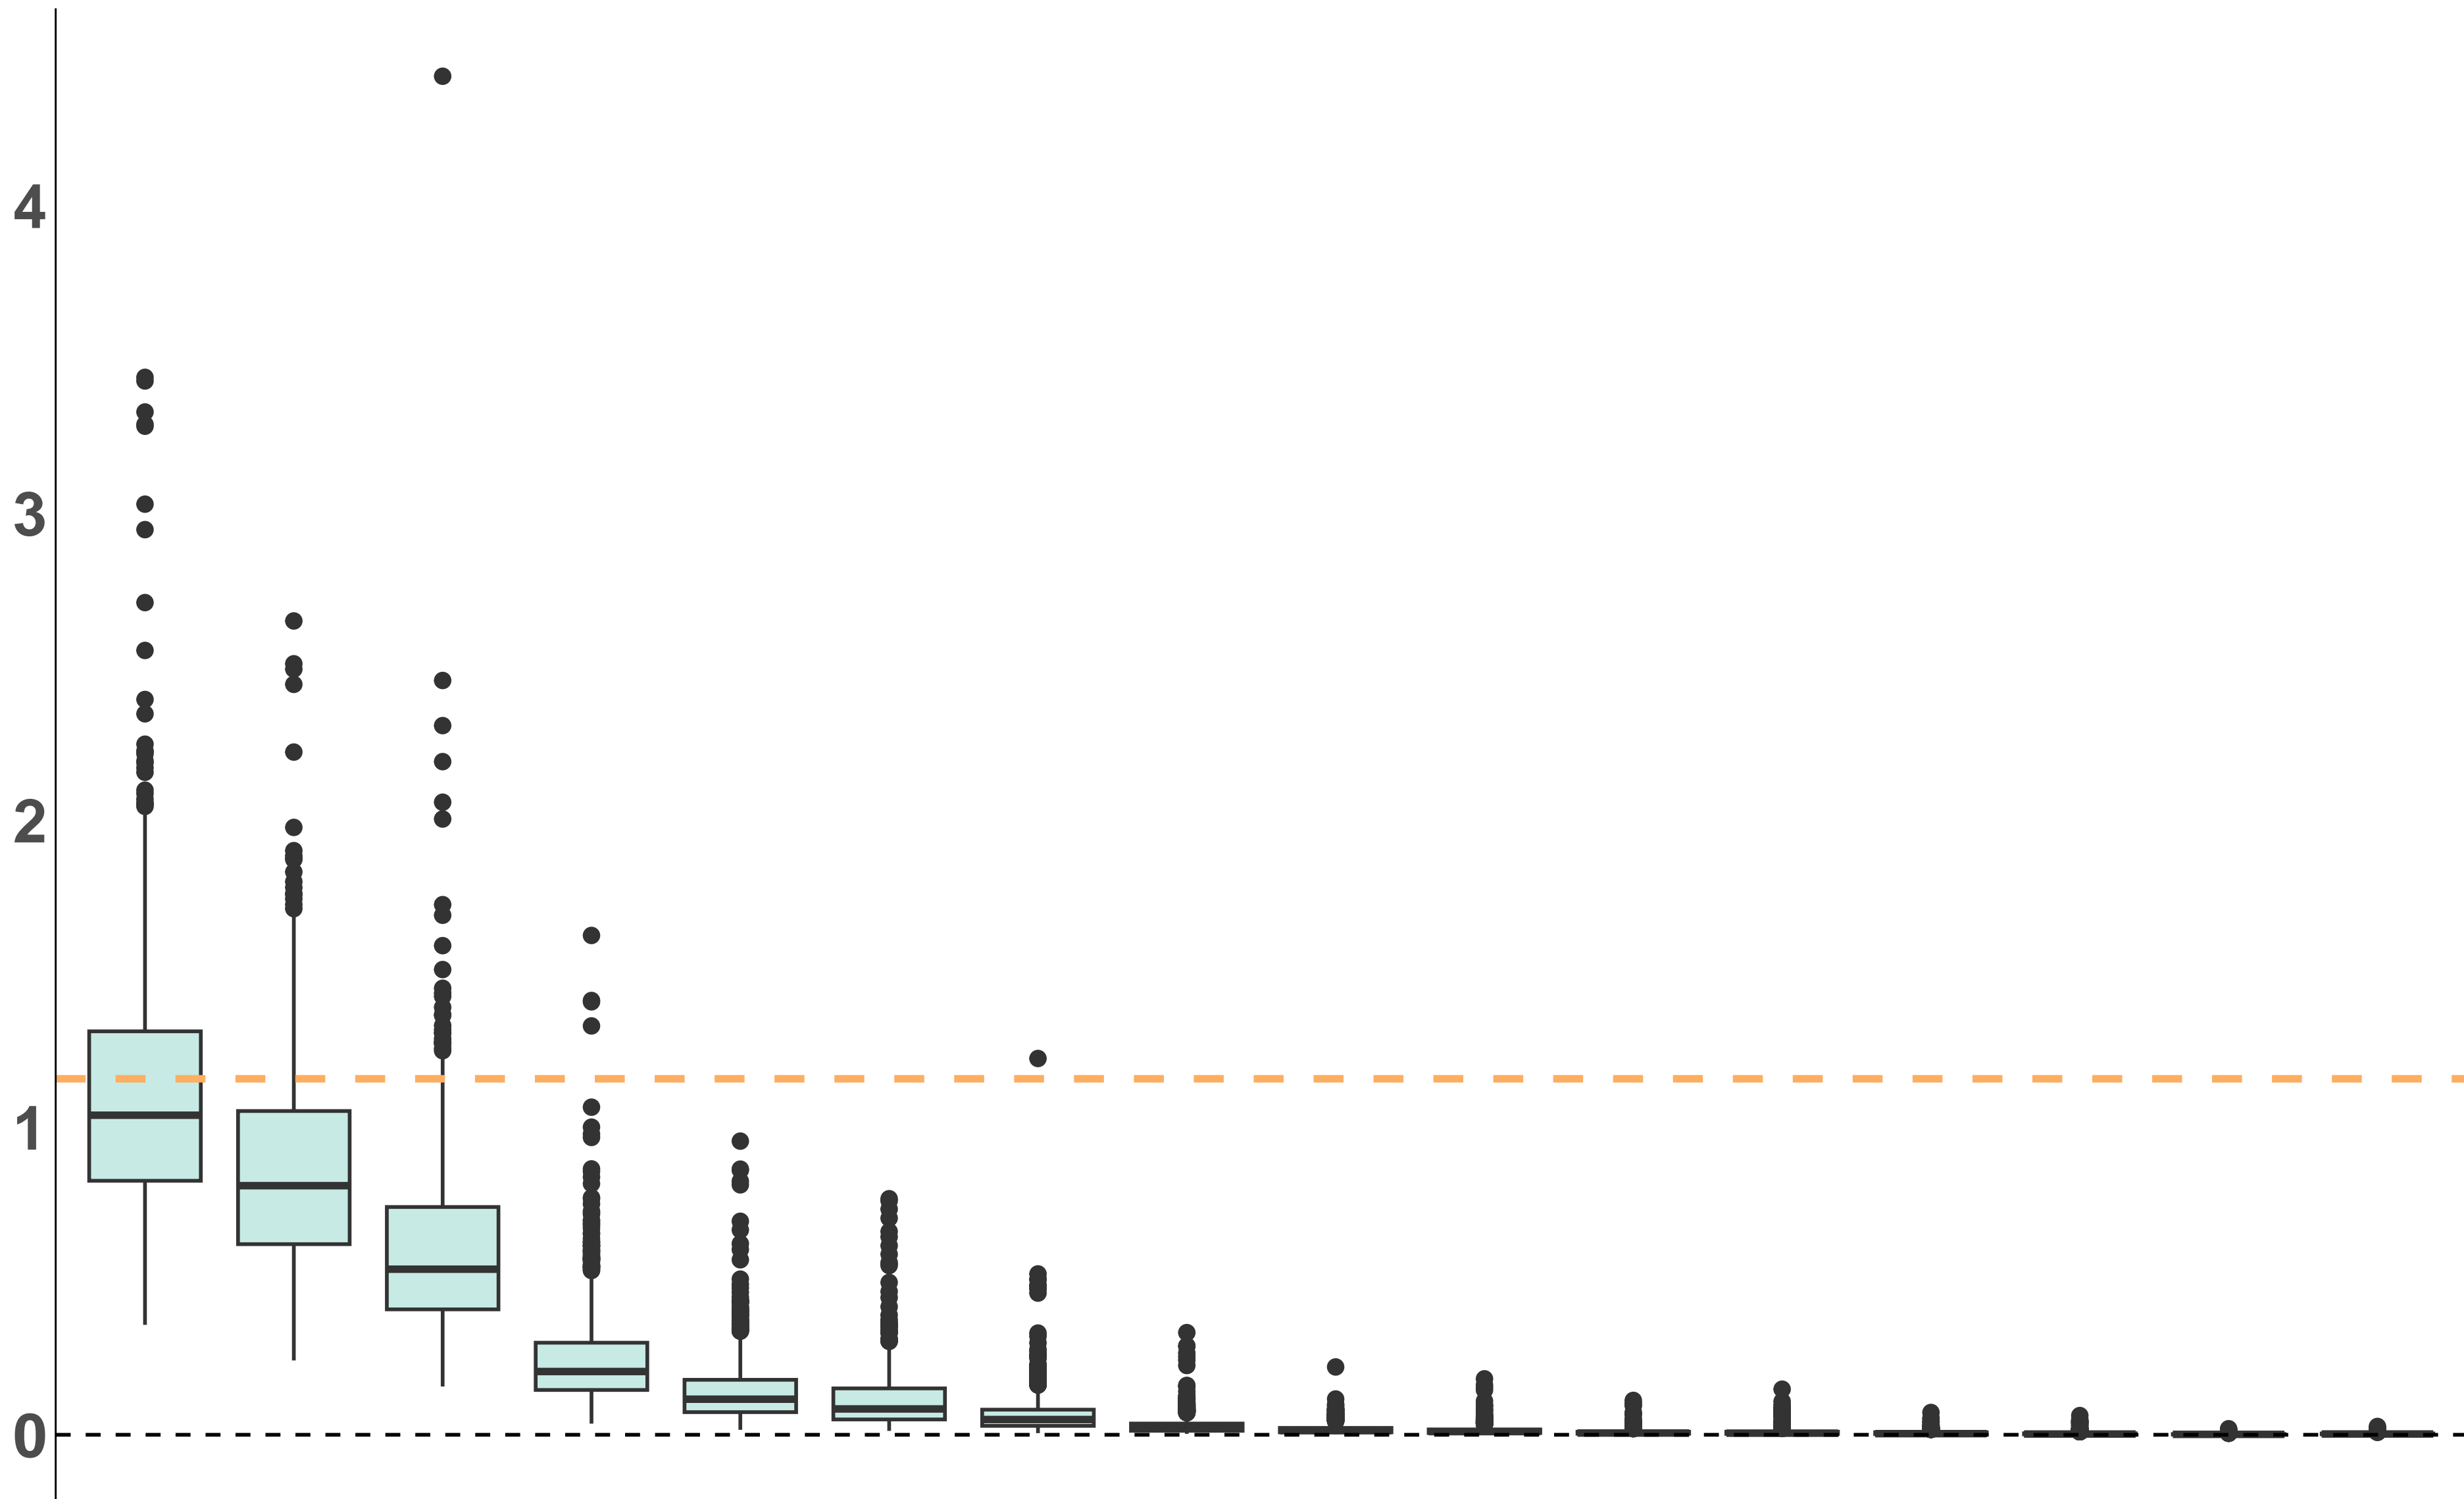

# RMSS

$\mu = 0.002$

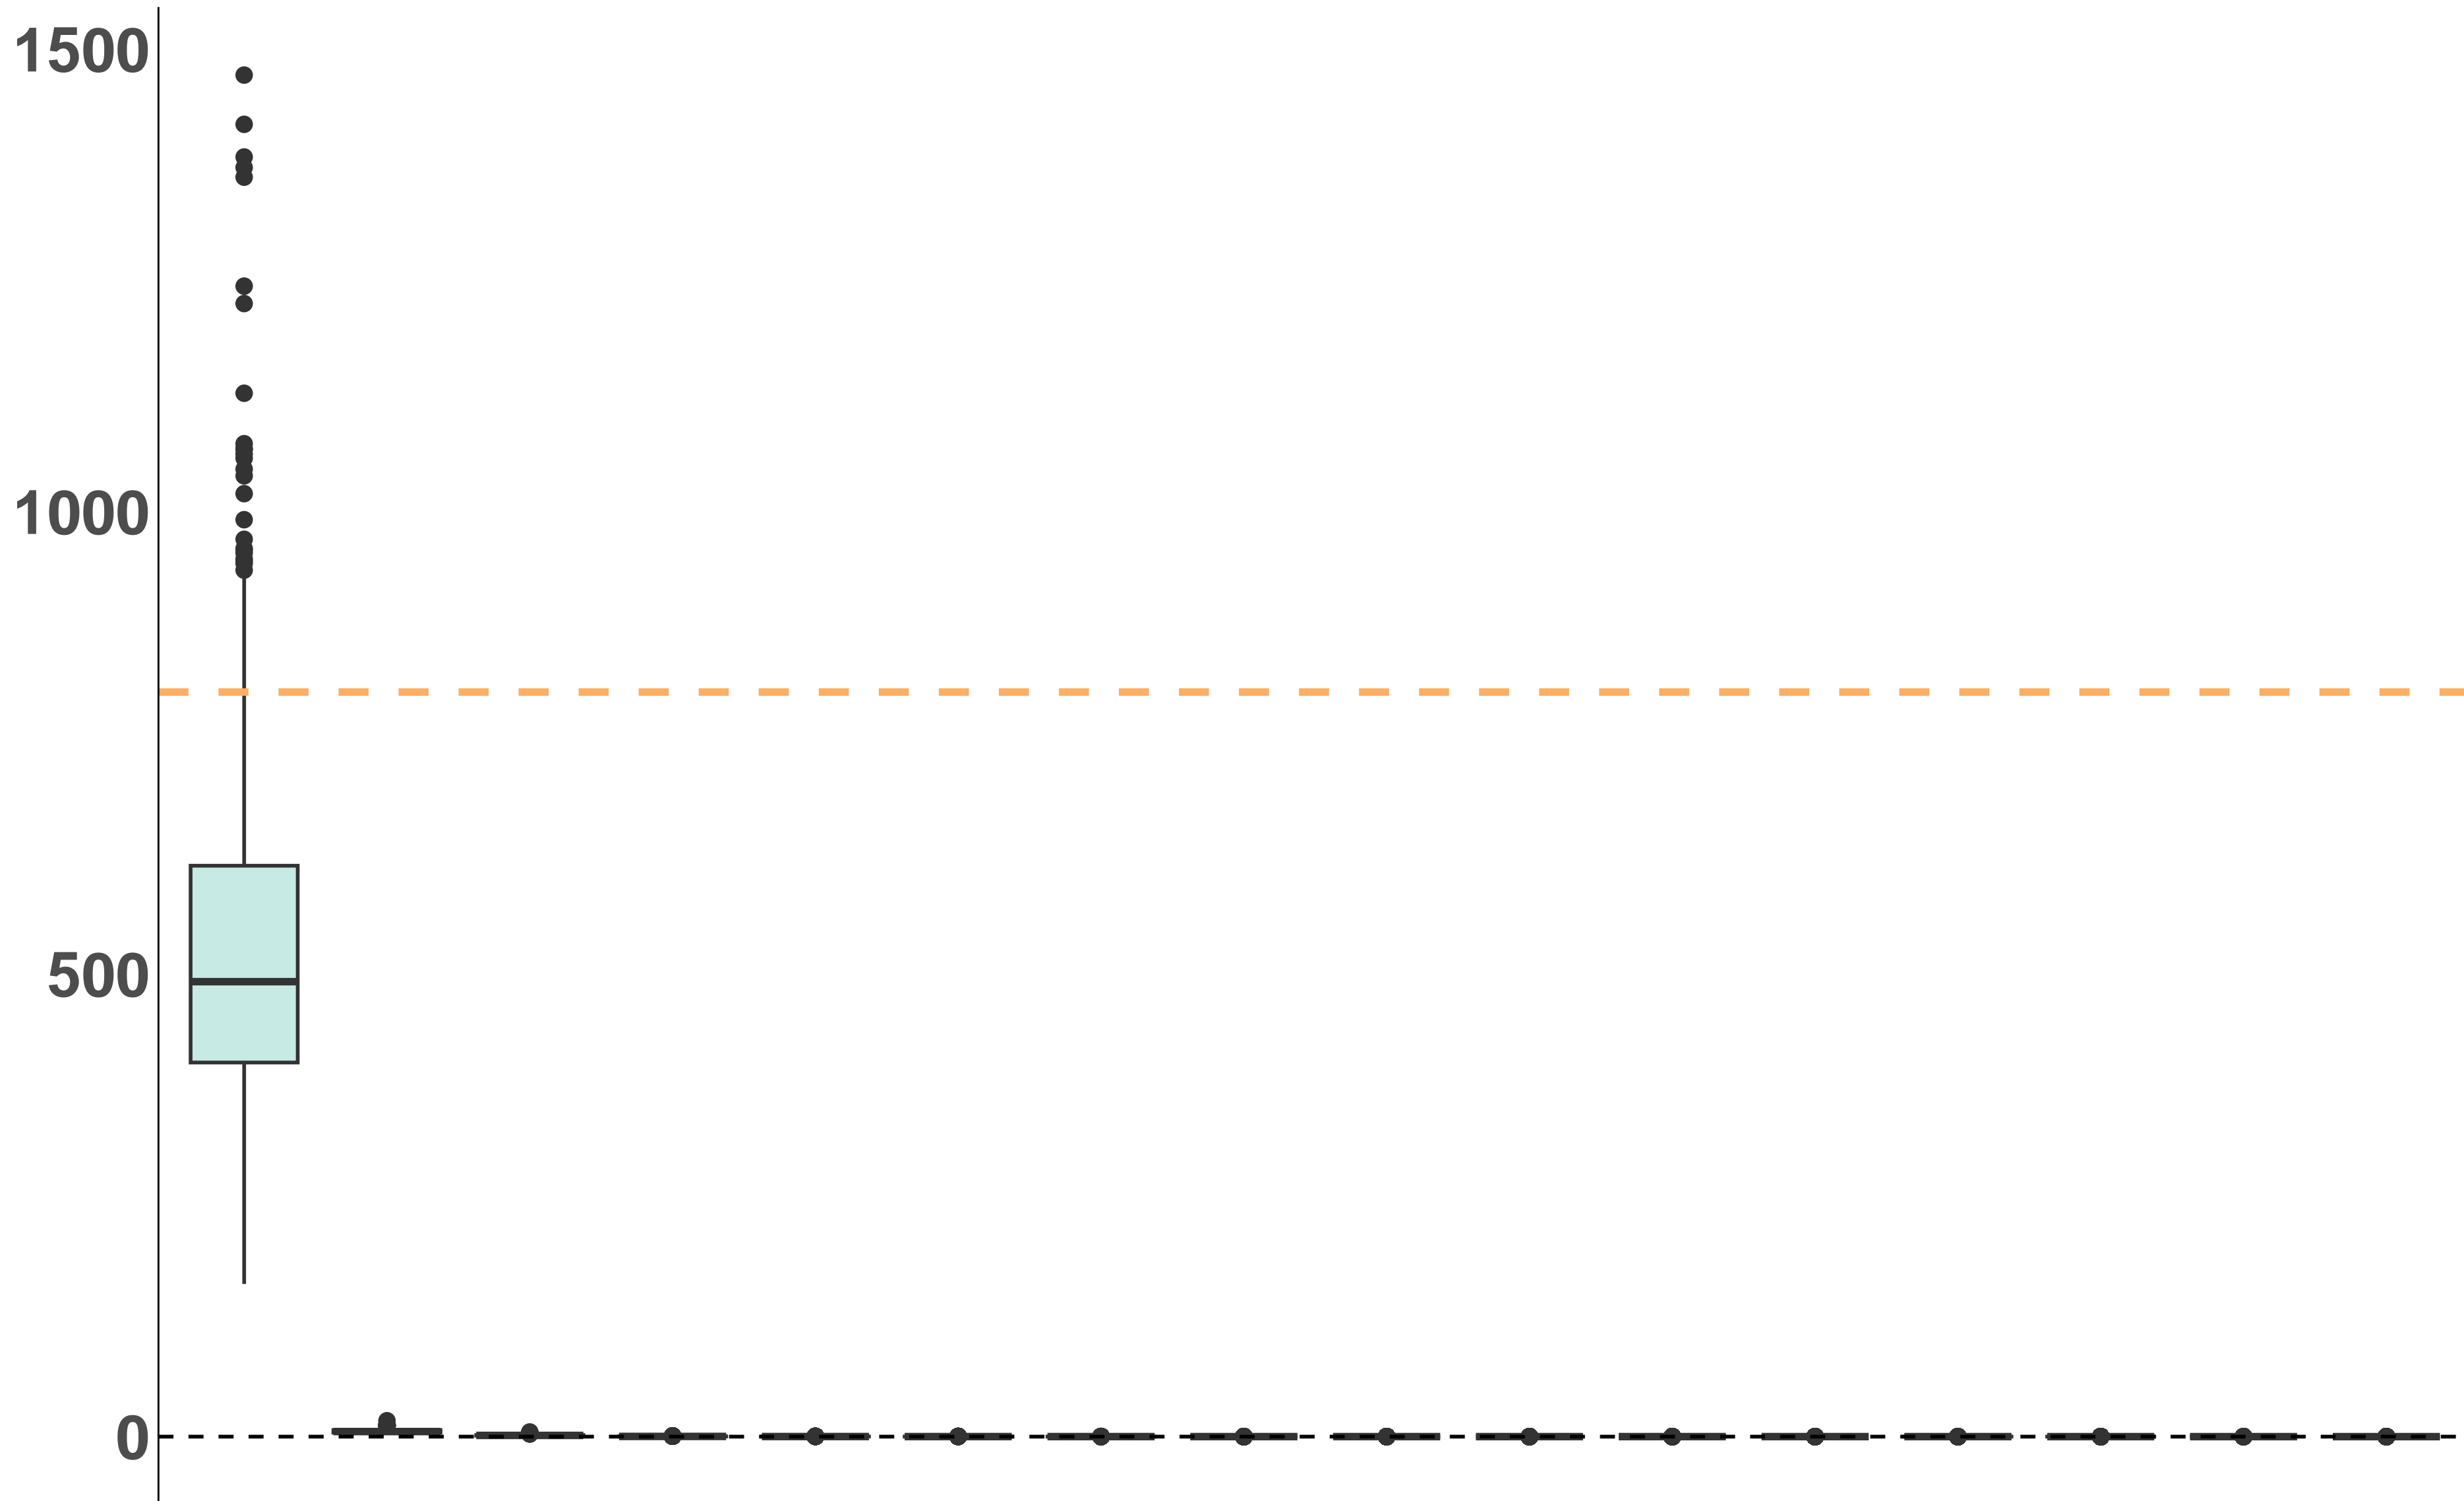

**mu = 0.02**

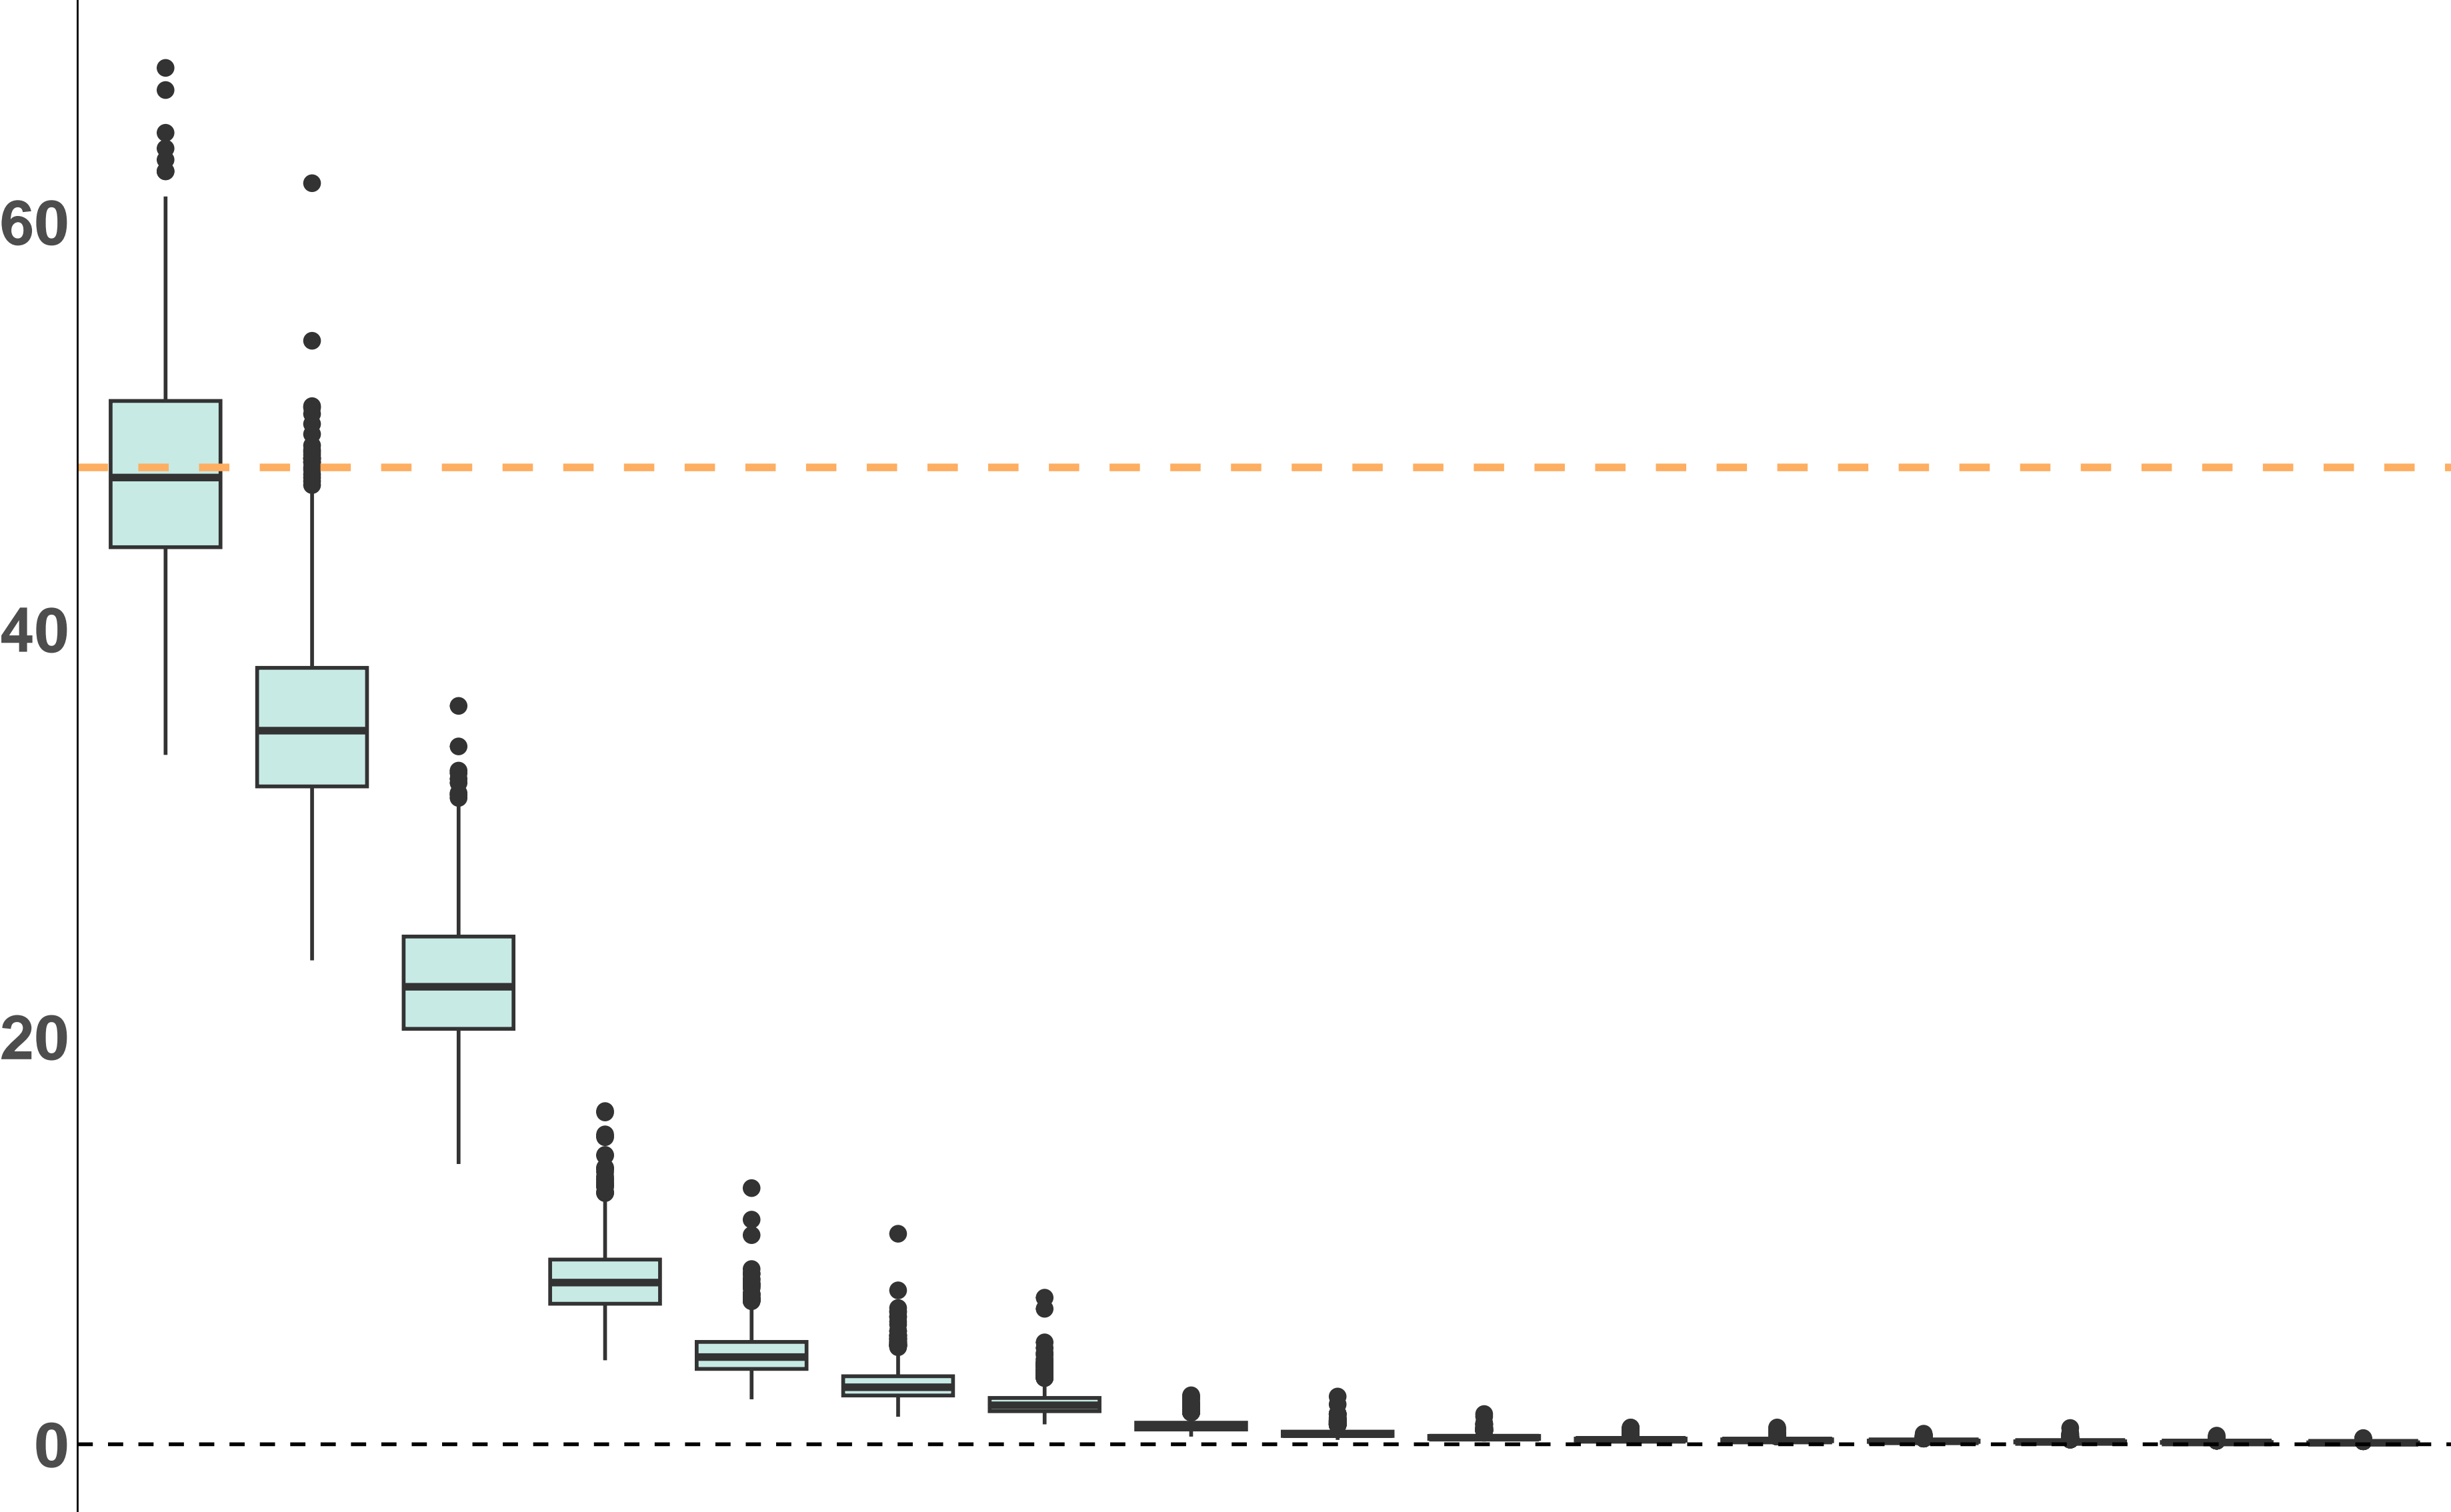

**mu = 0.02**

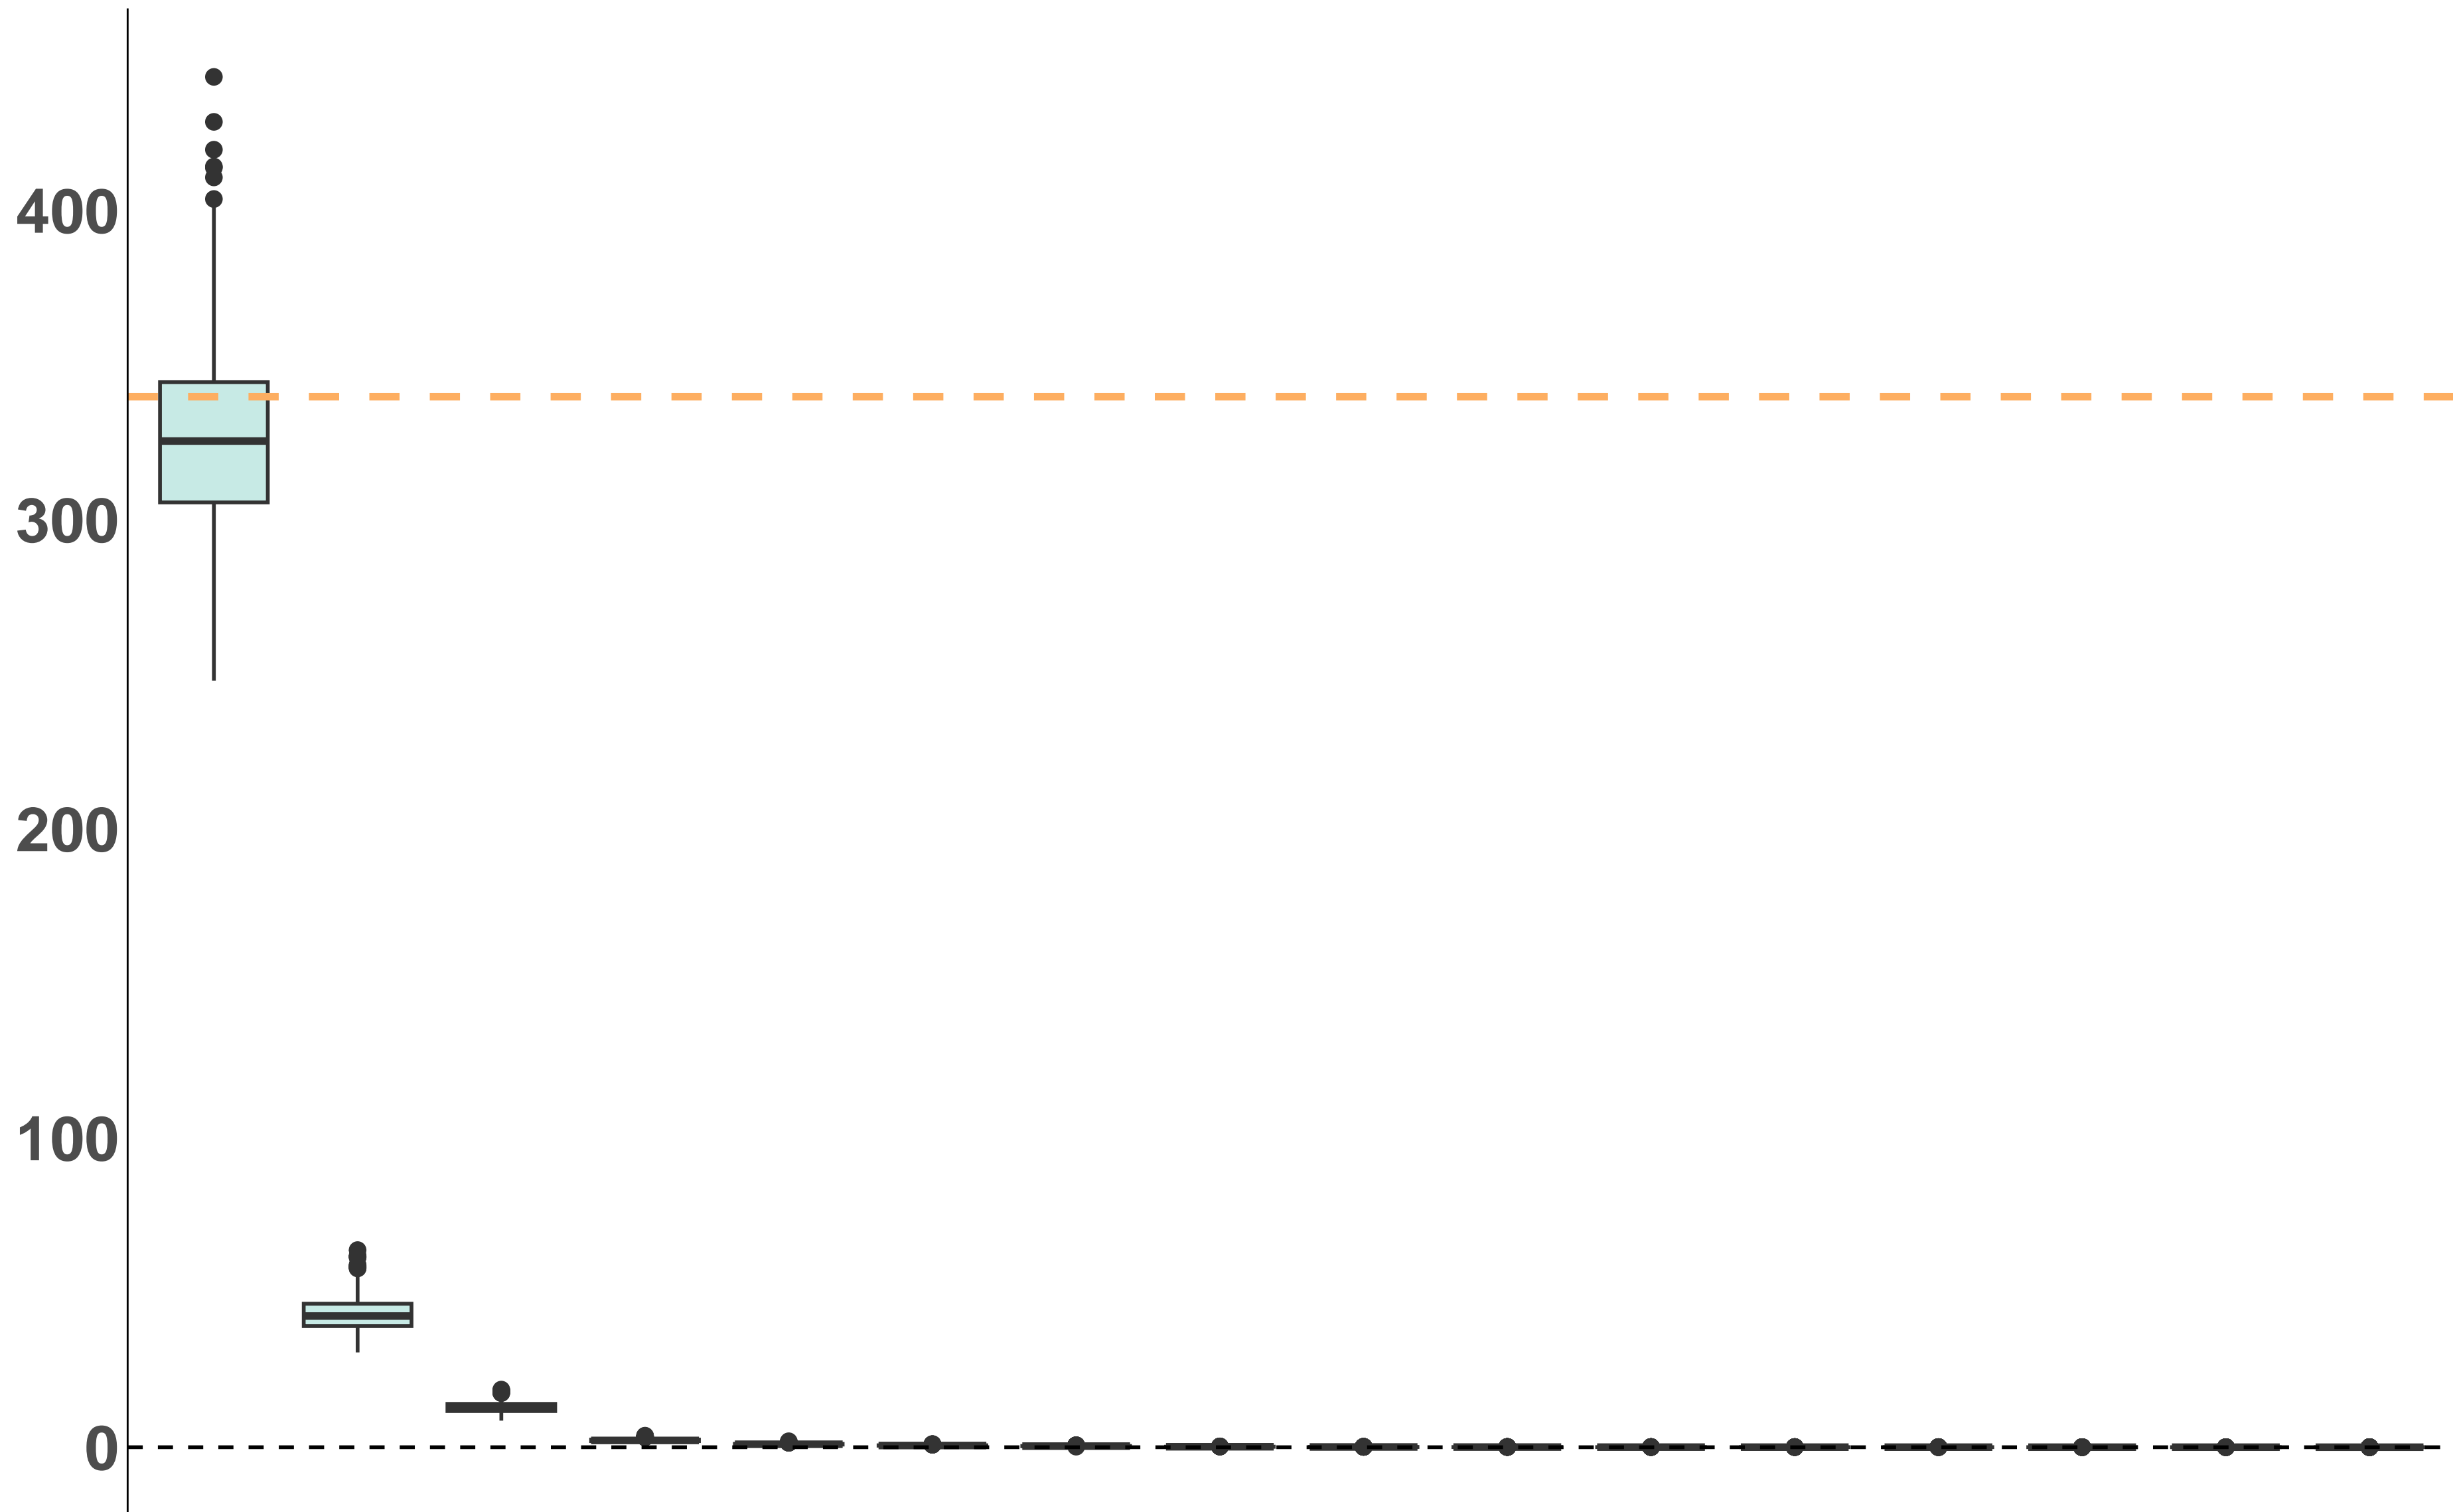

**mu = 0.2**

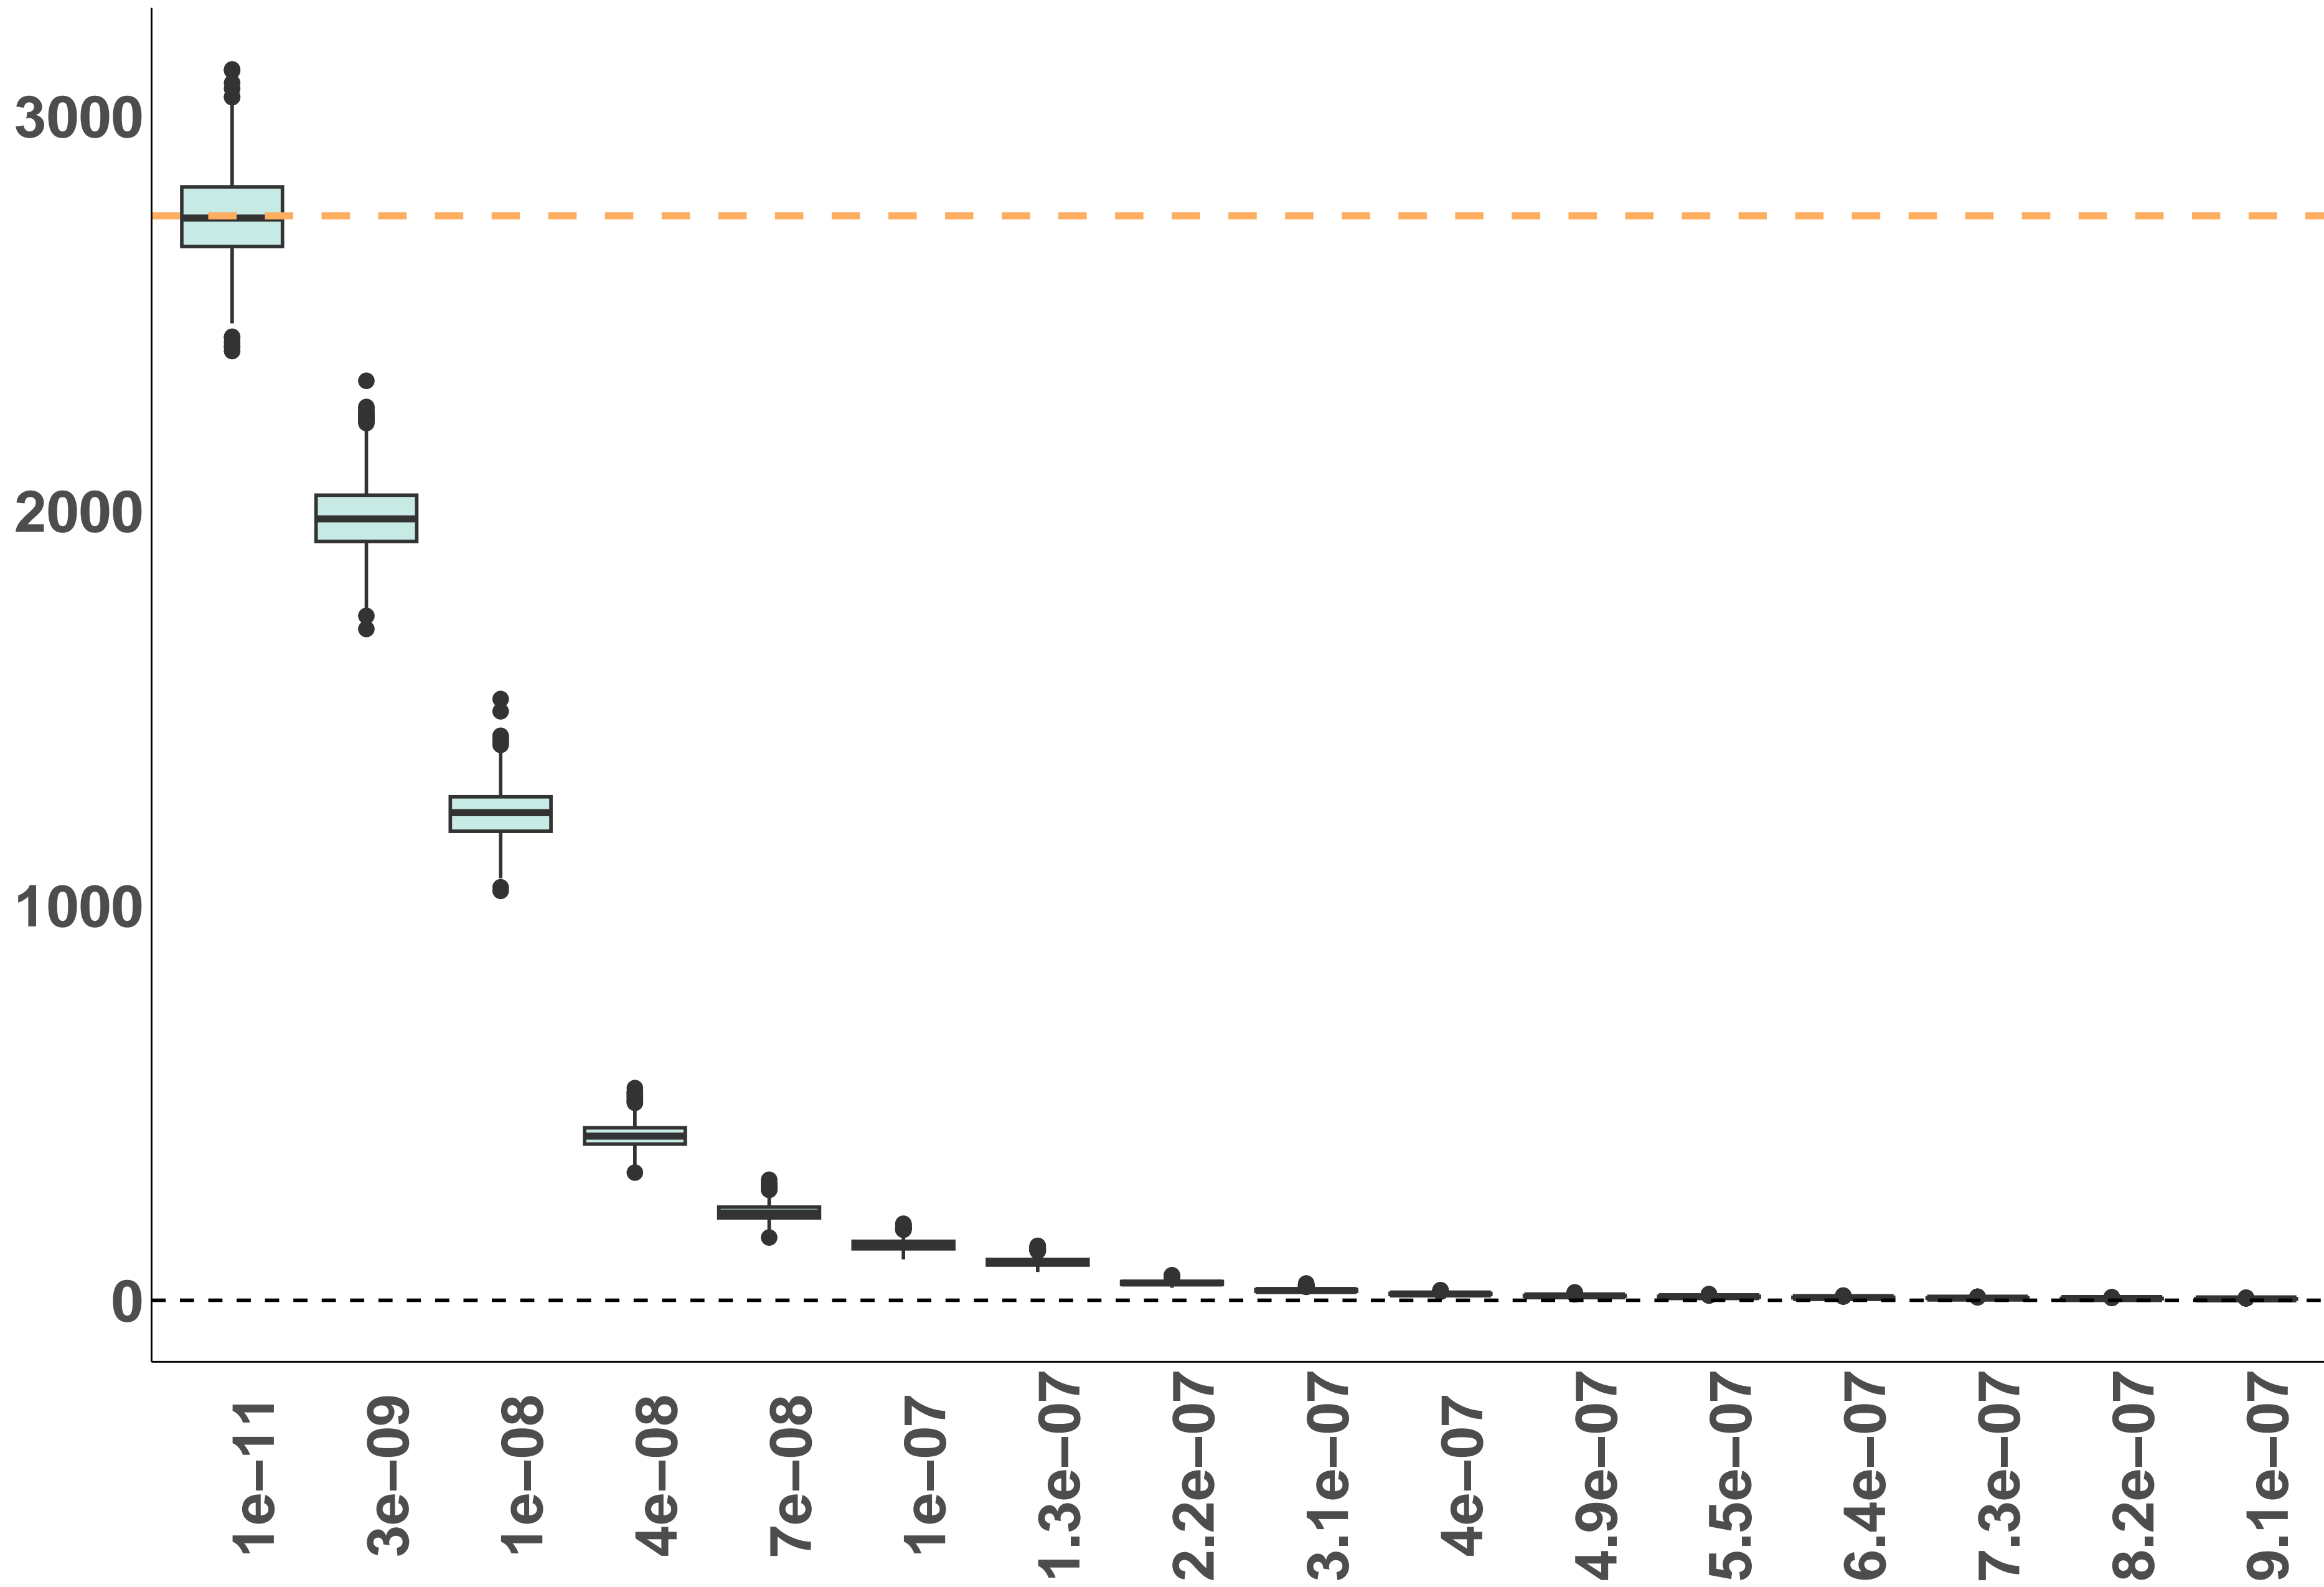

**mu = 0.2**

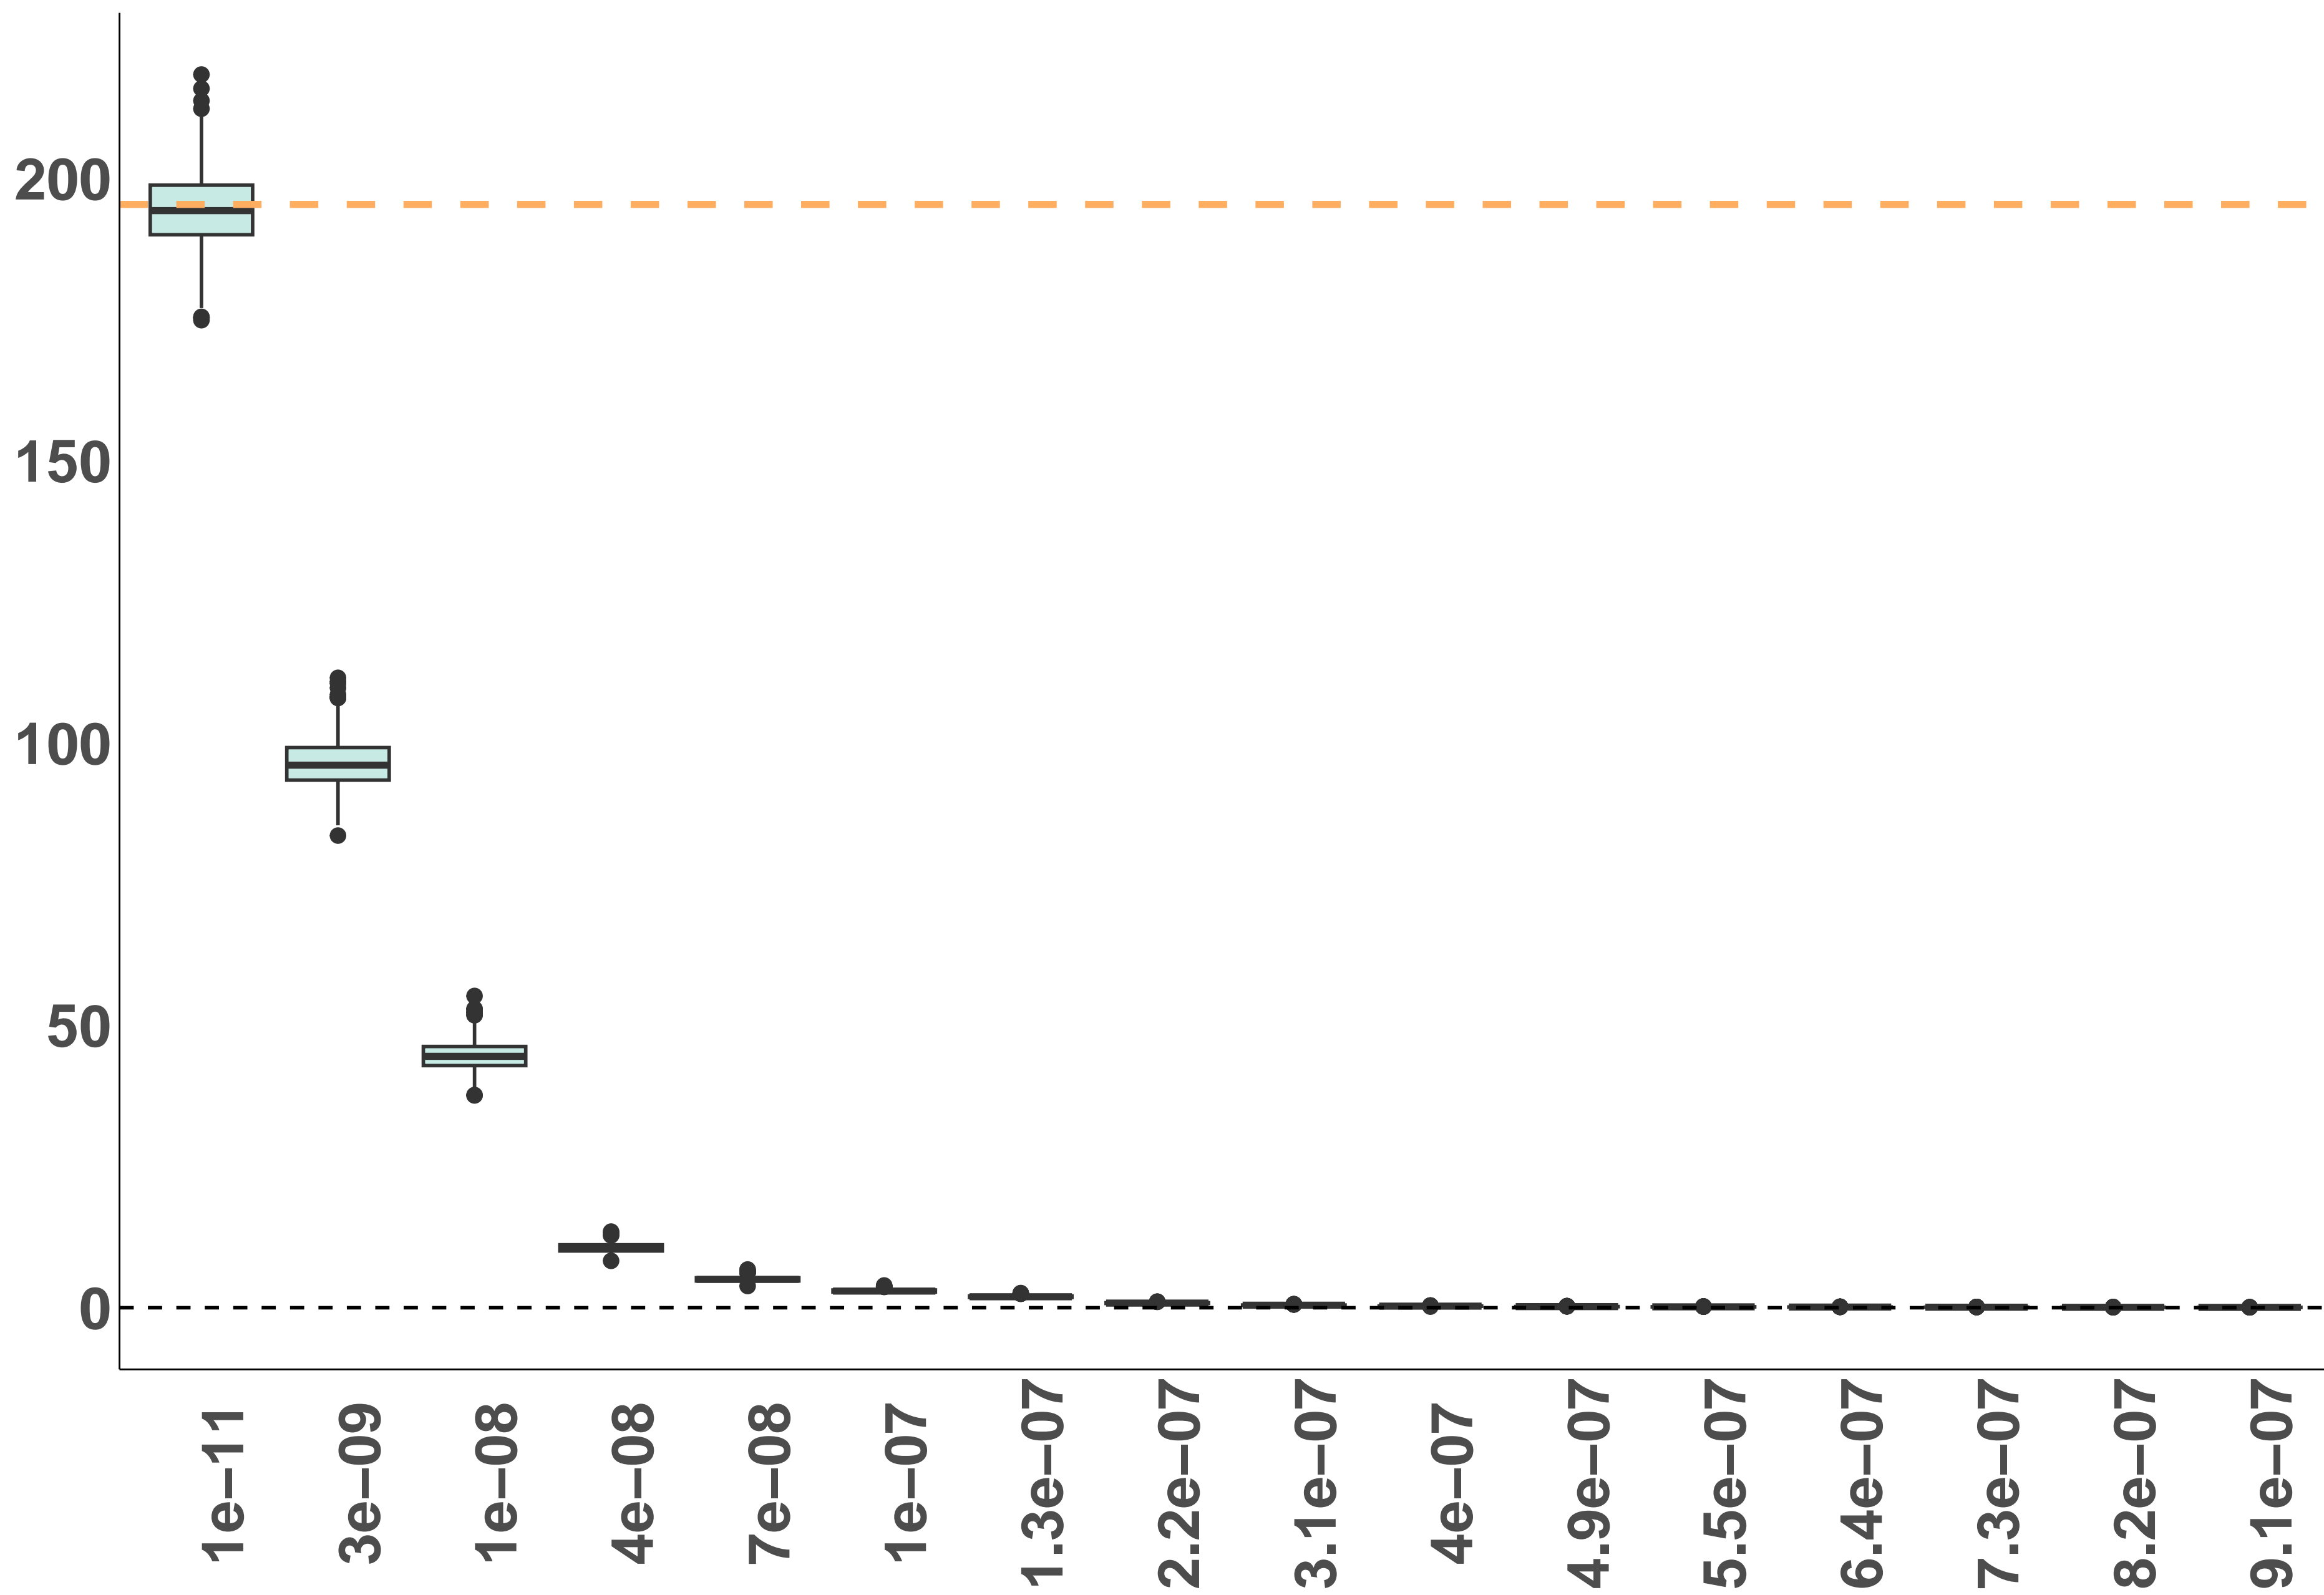

Supplement: Supplementary file 1 [file FigureA1.pdf]
