# Supplementary material for: On prior smoothing with discrete spatial data in the context of disease mapping
Source: arXiv:2503.16151 source file (2025-07-29)

# max MSS

$\mu = 0.002$

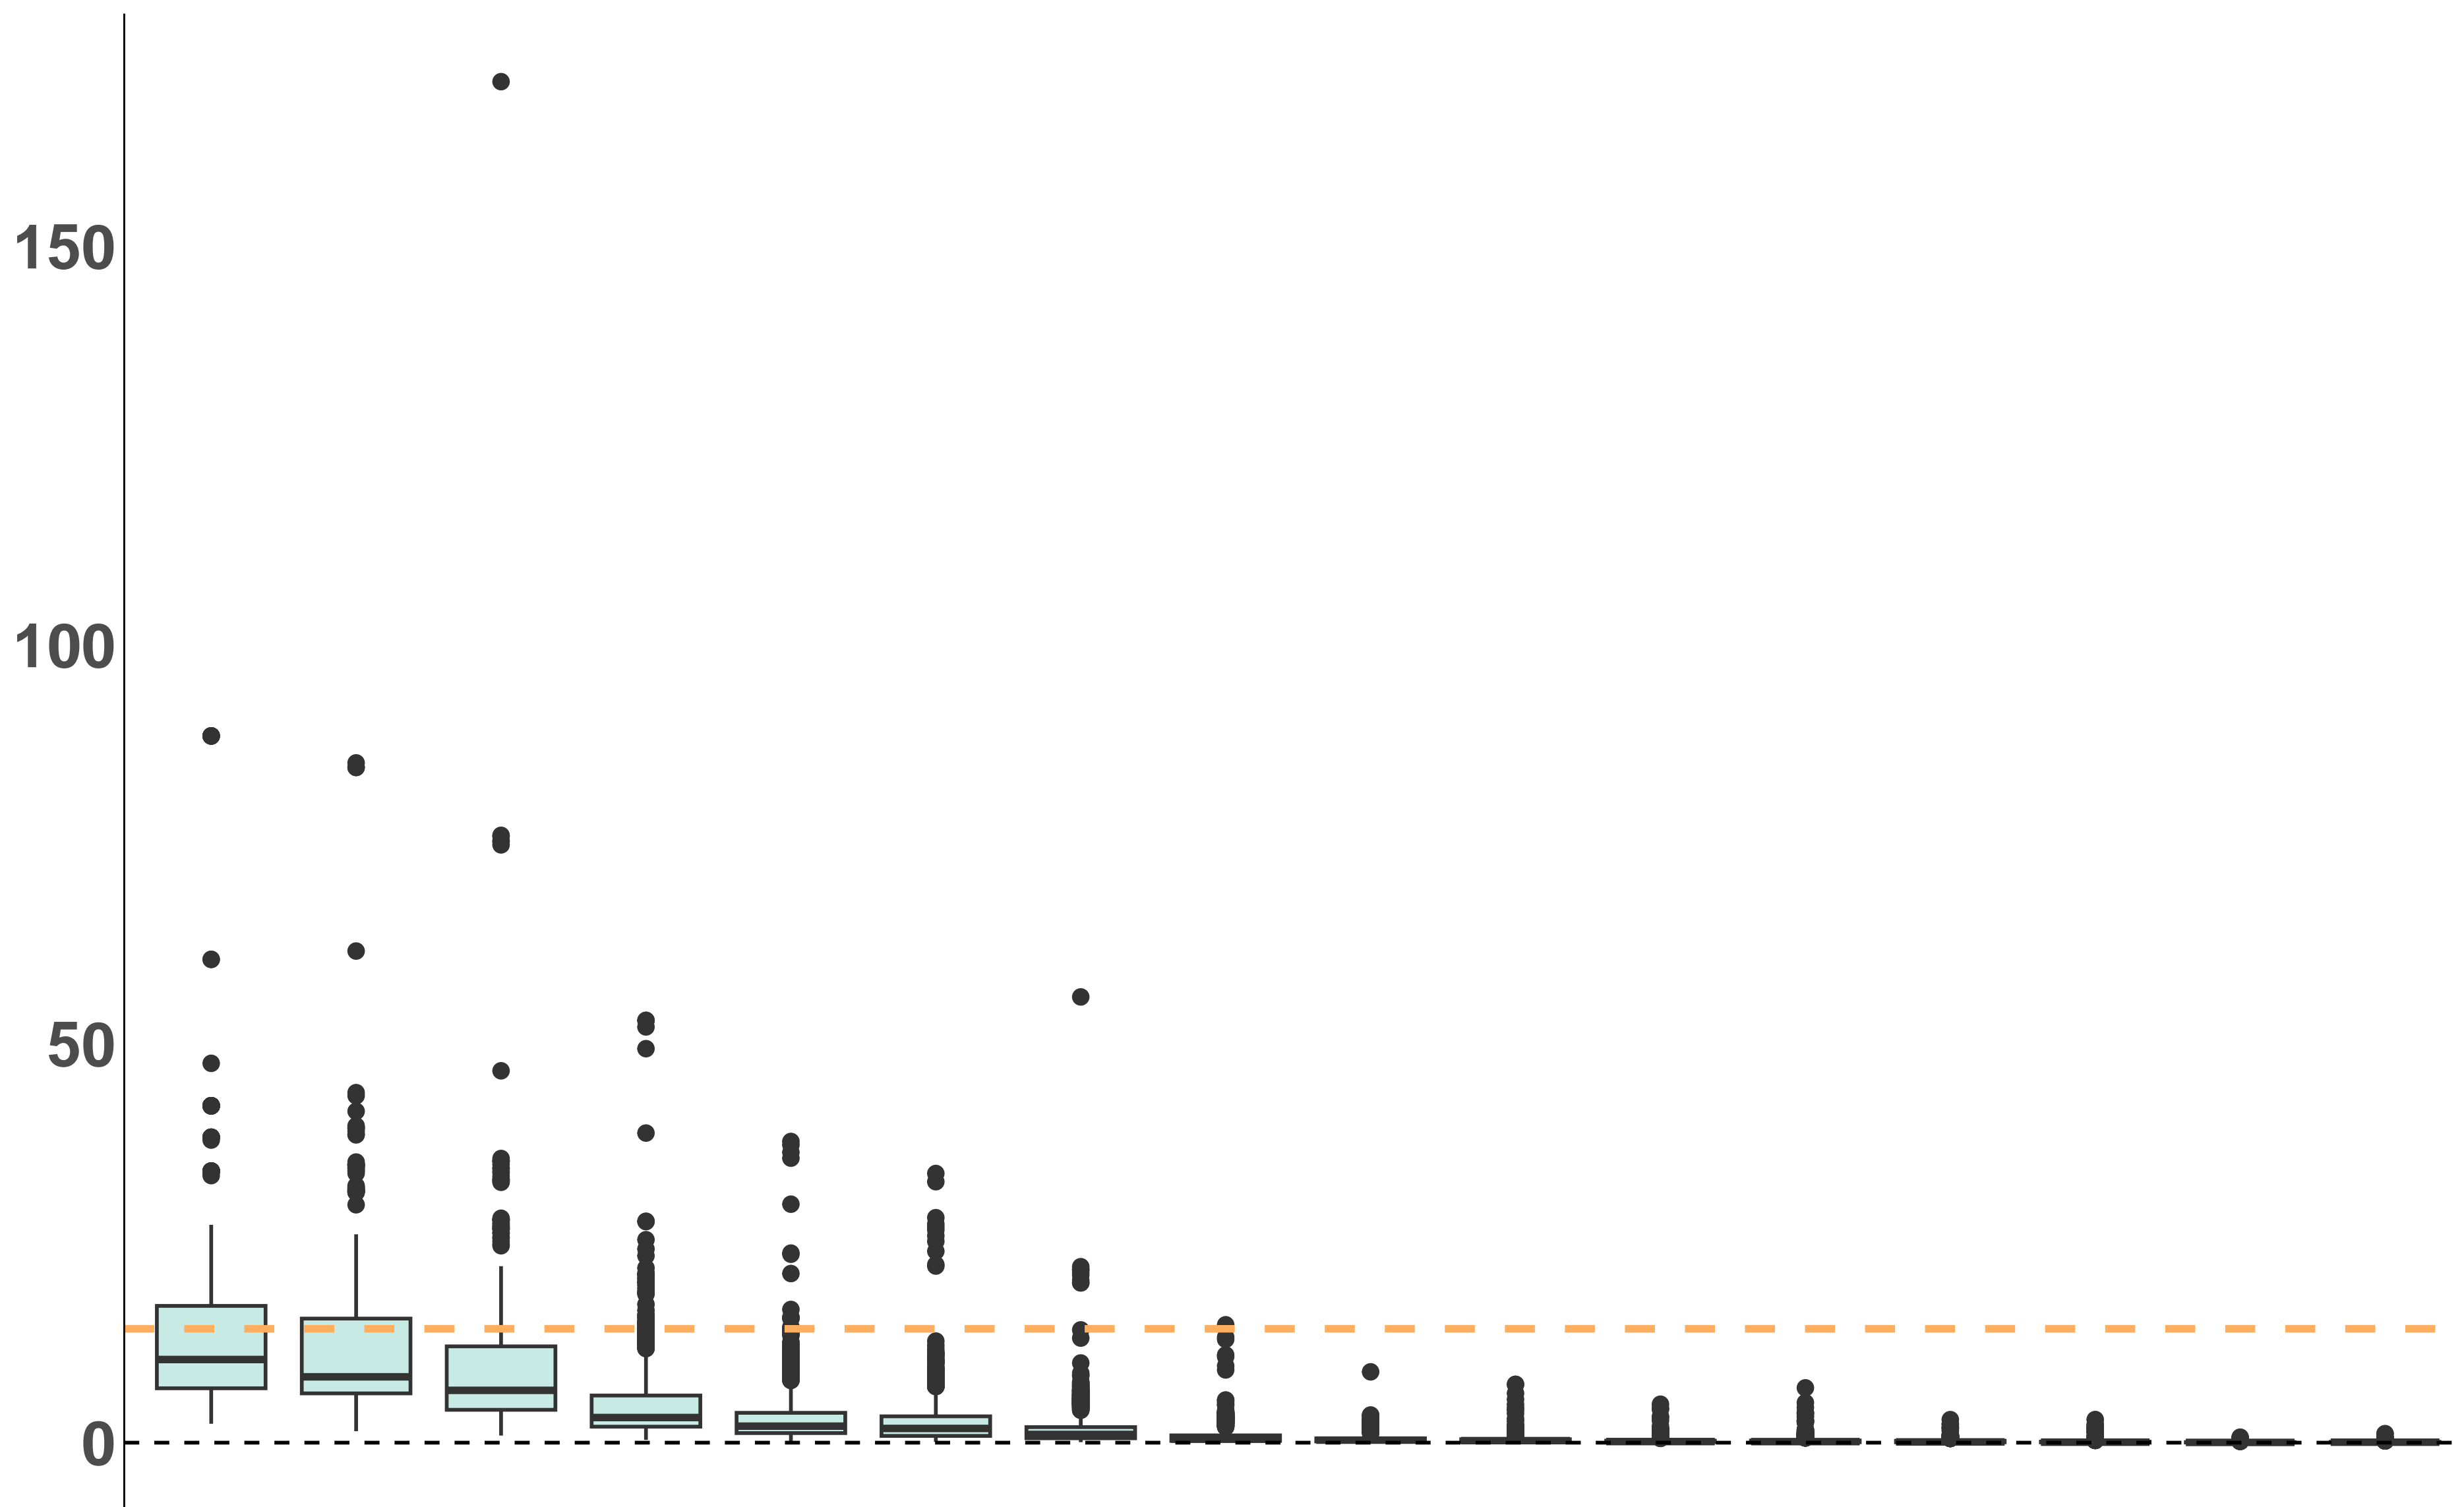

# max RMSS

$\mu = 0.002$

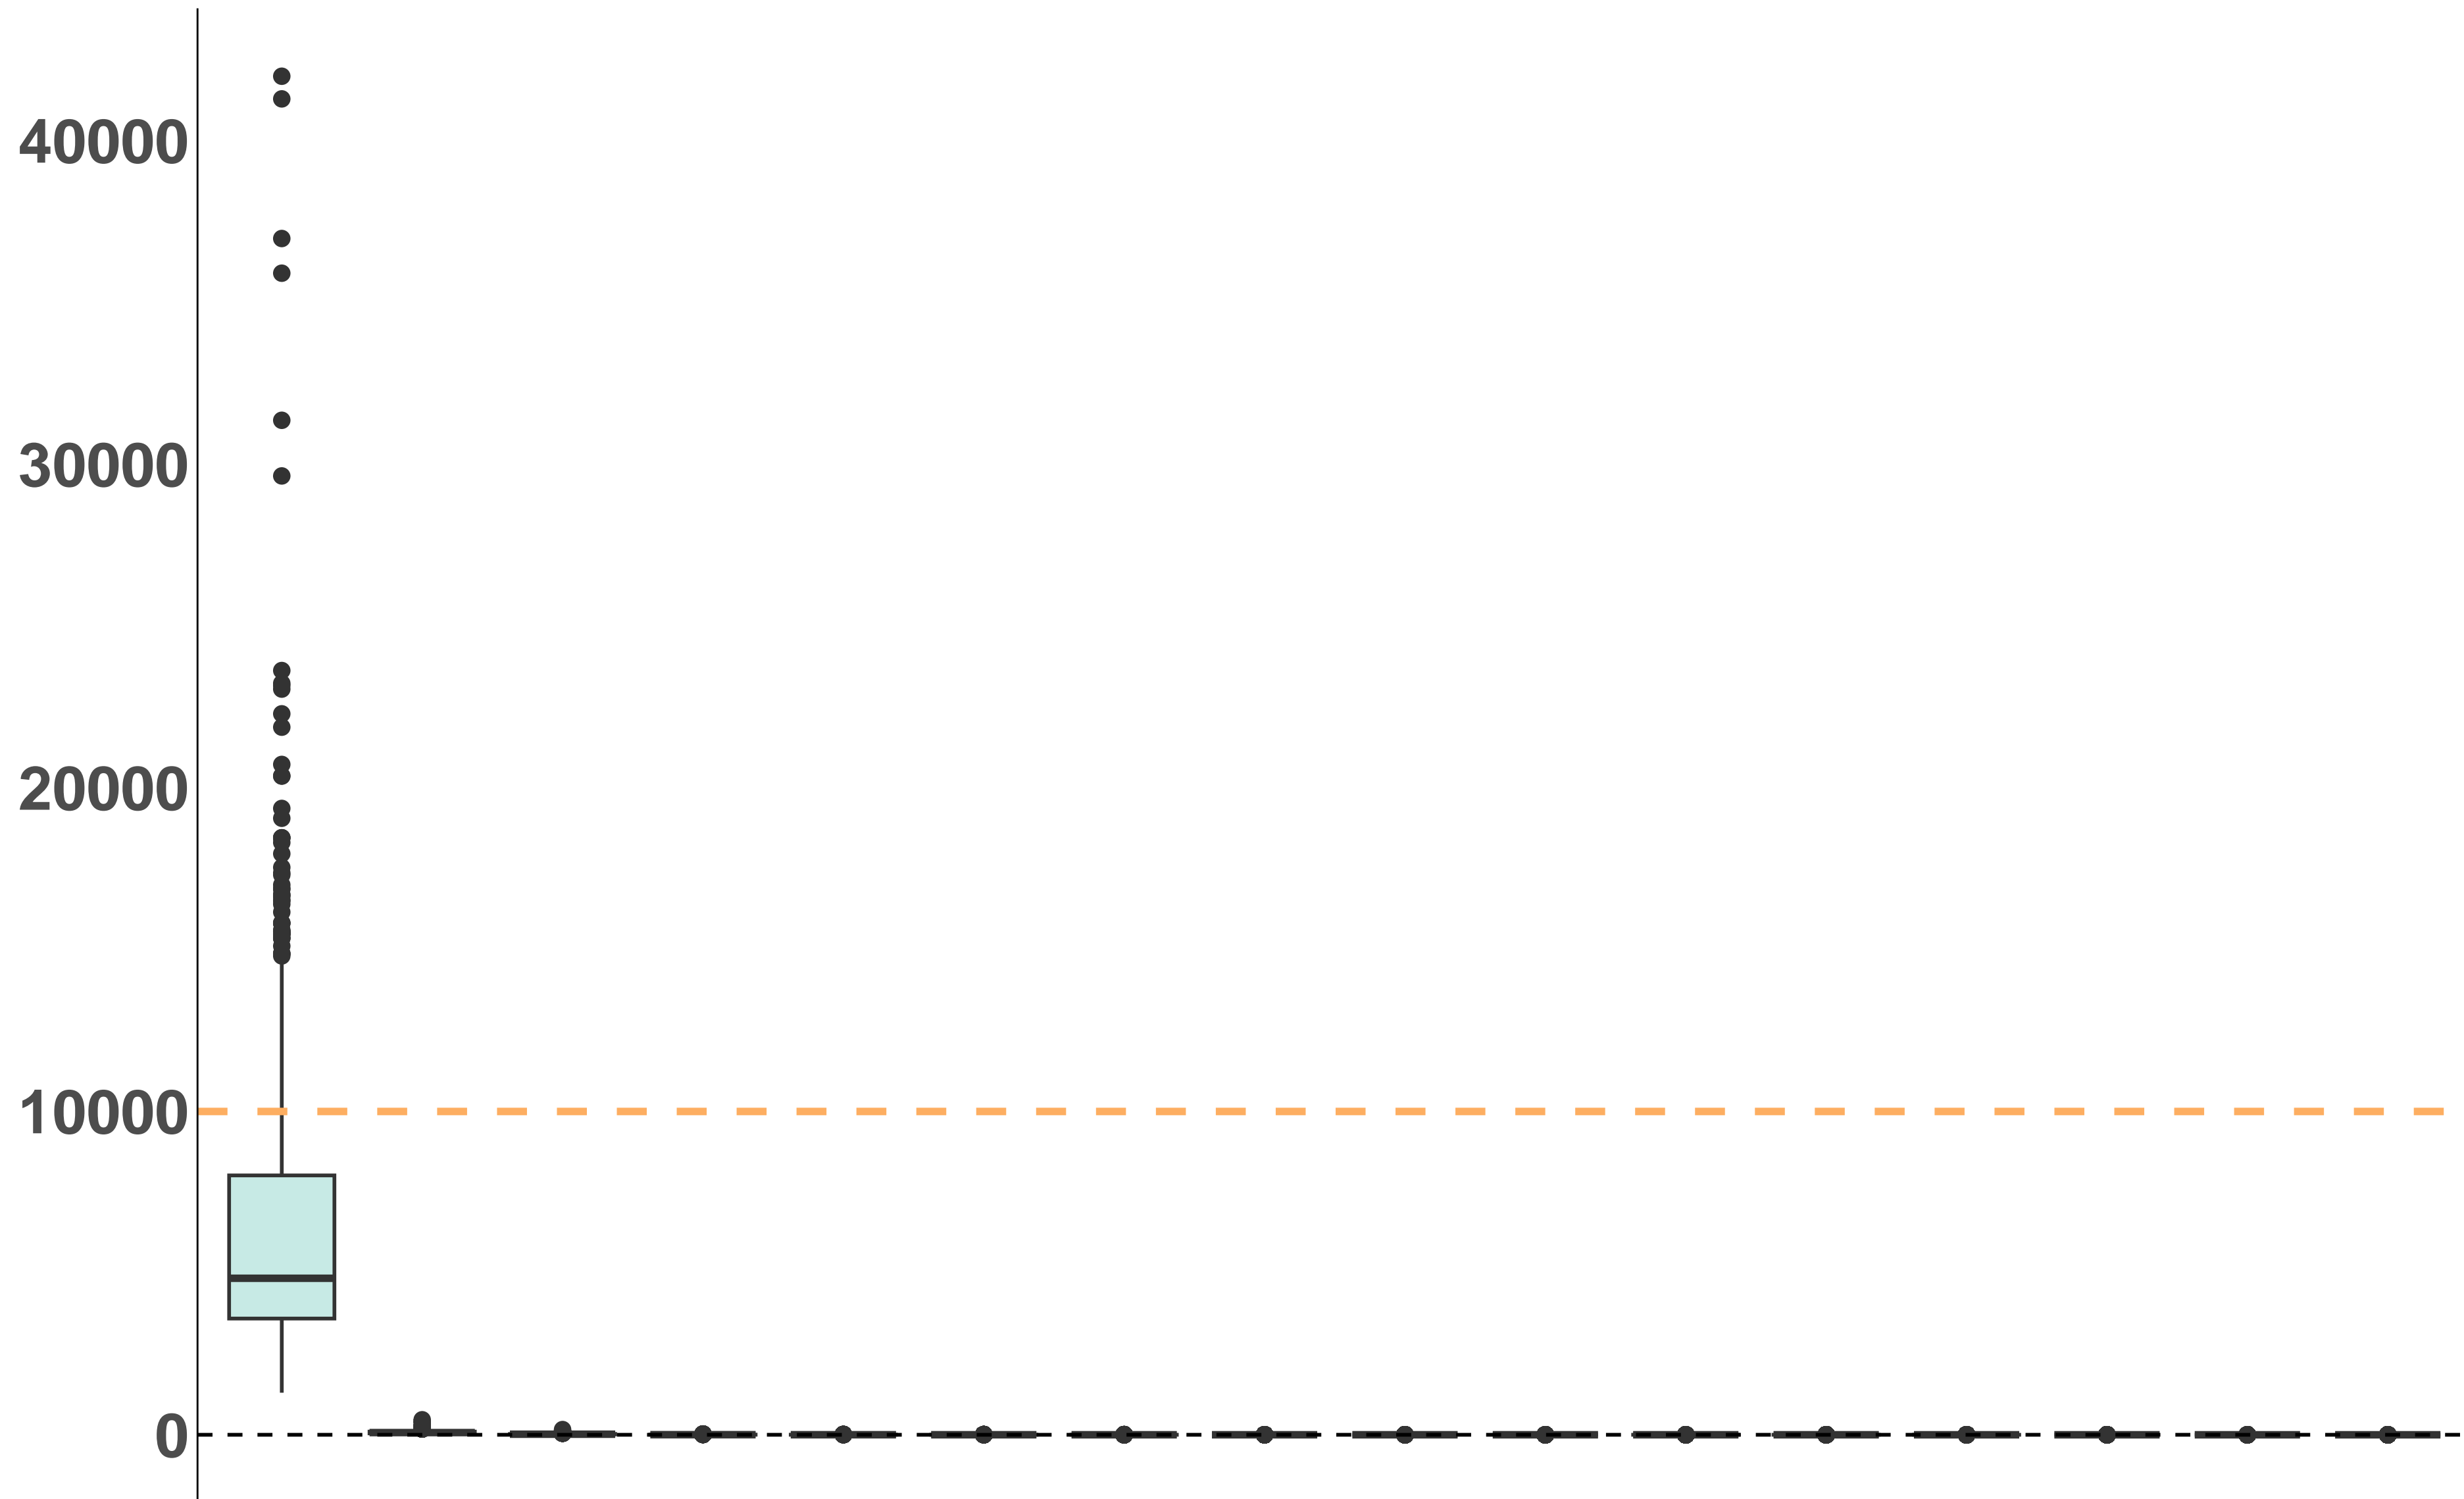

**mu = 0.02**

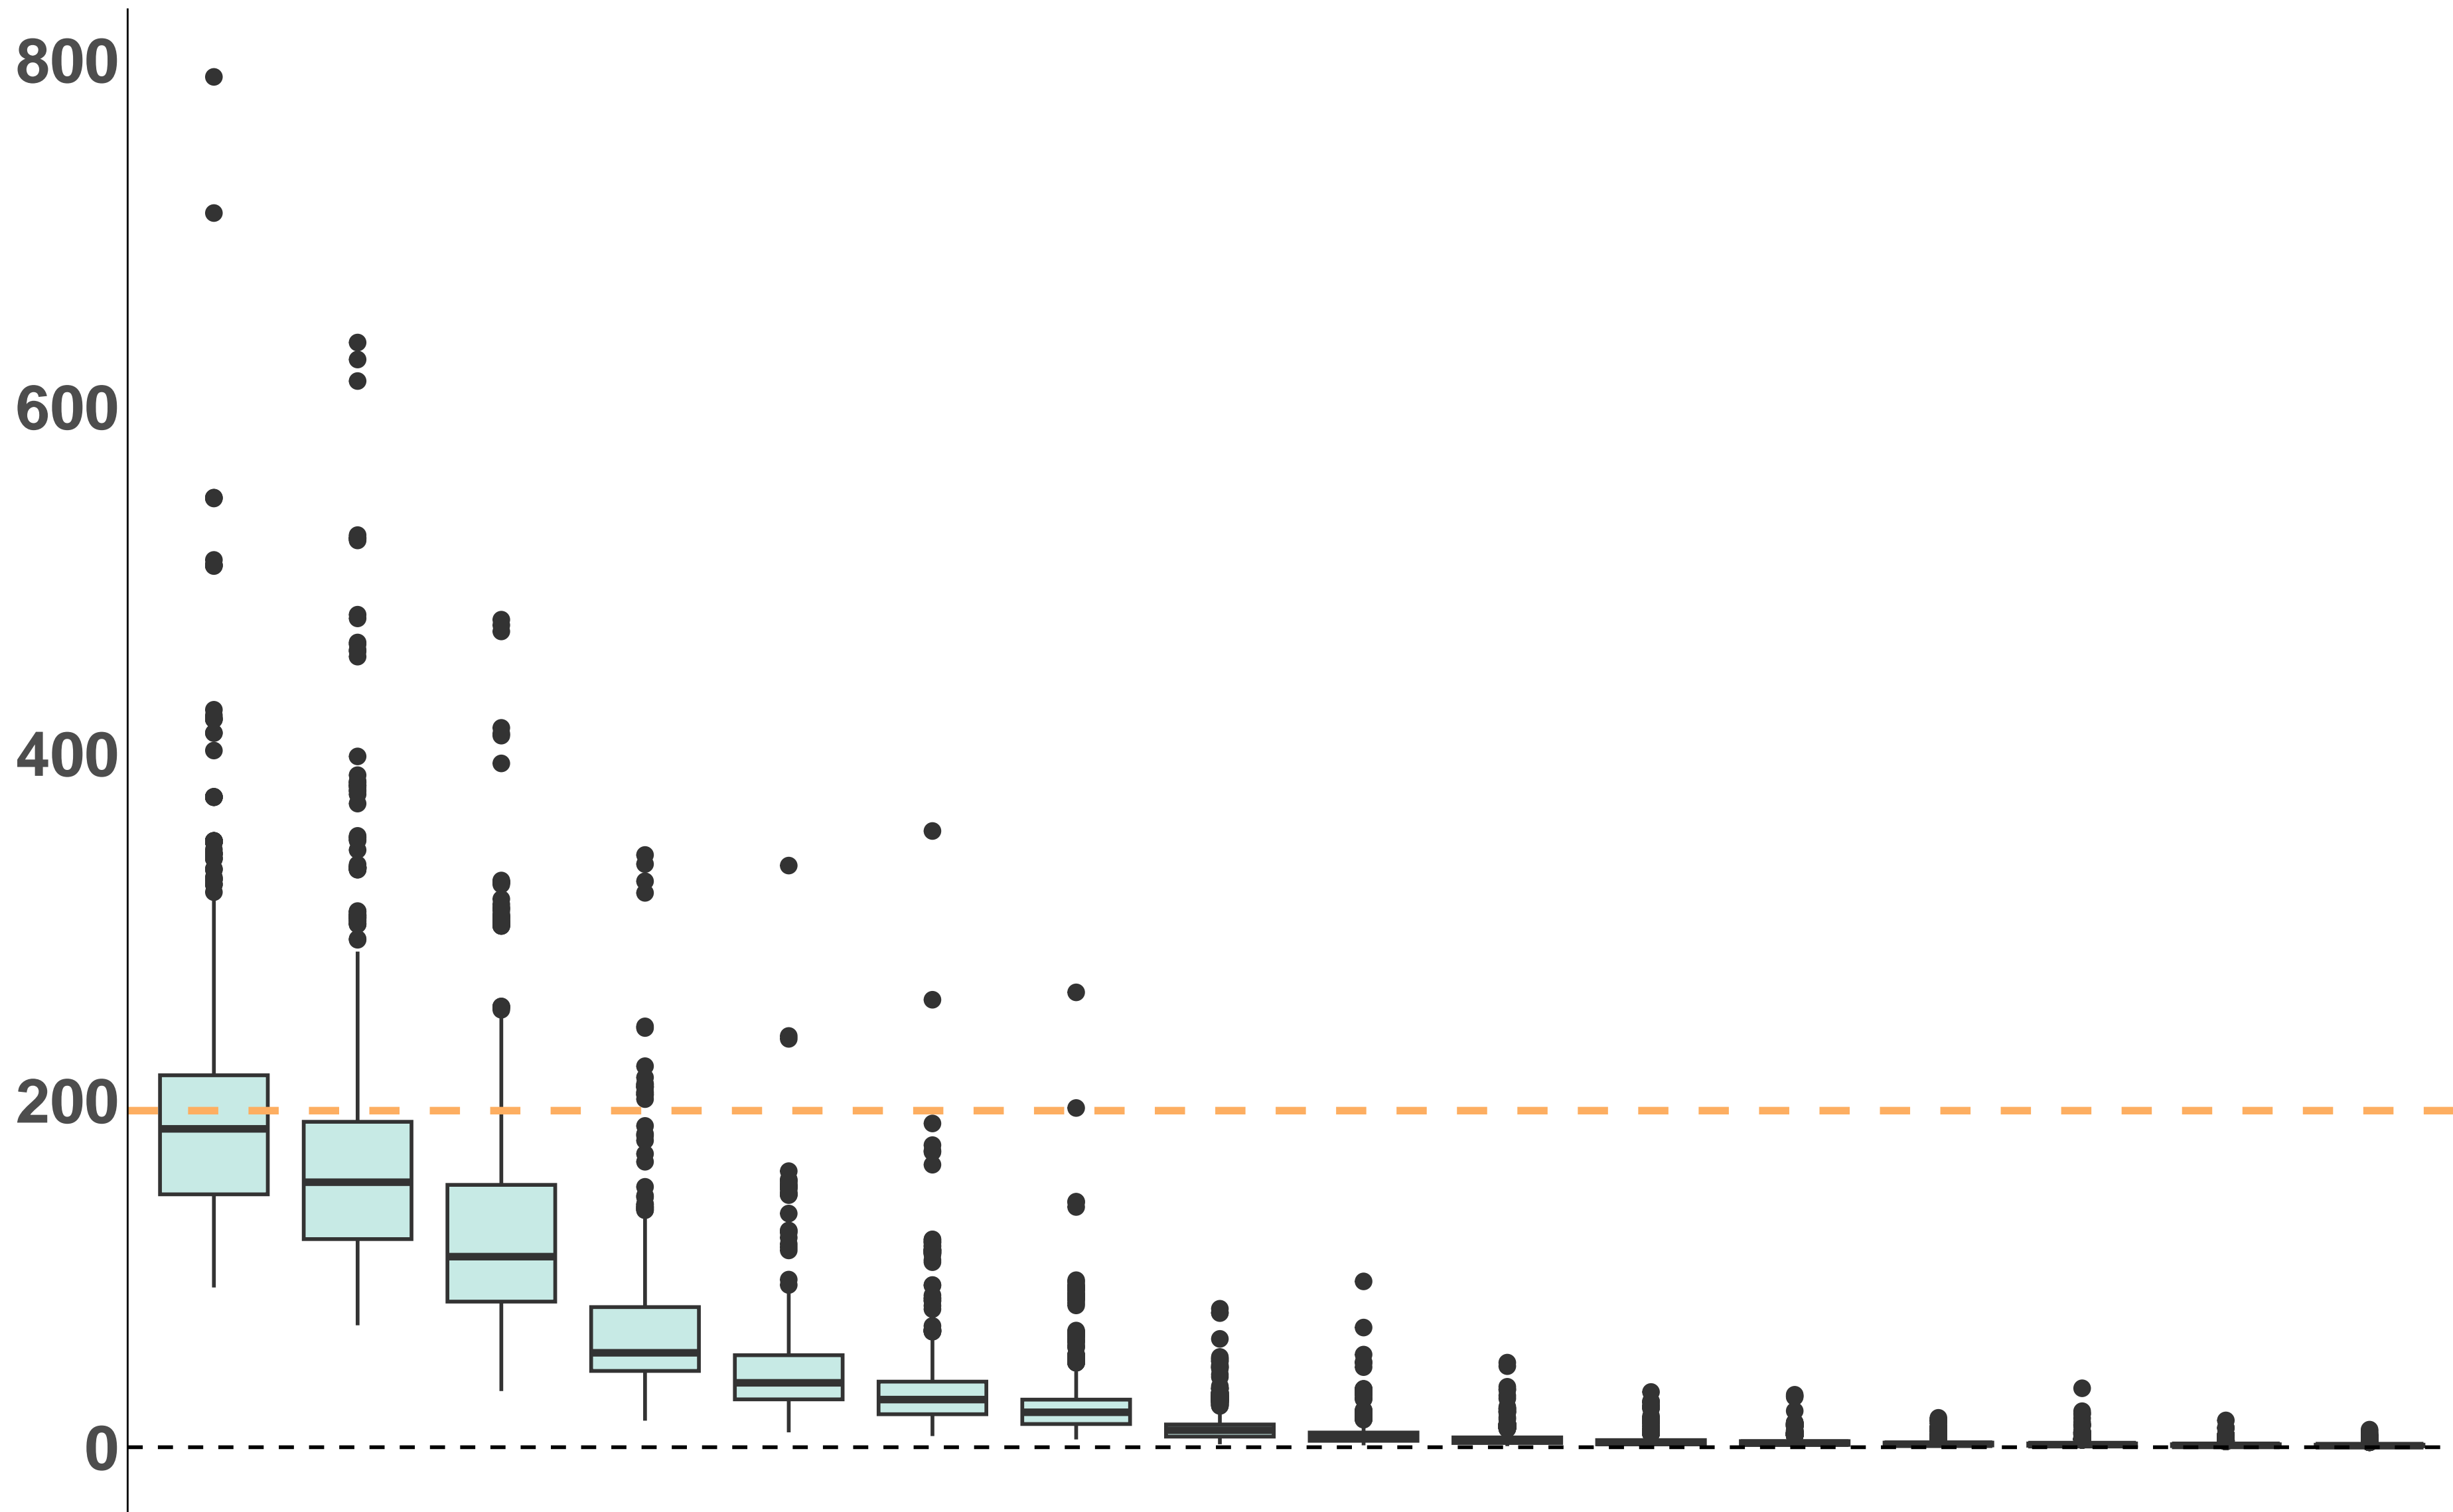

**mu = 0.02**

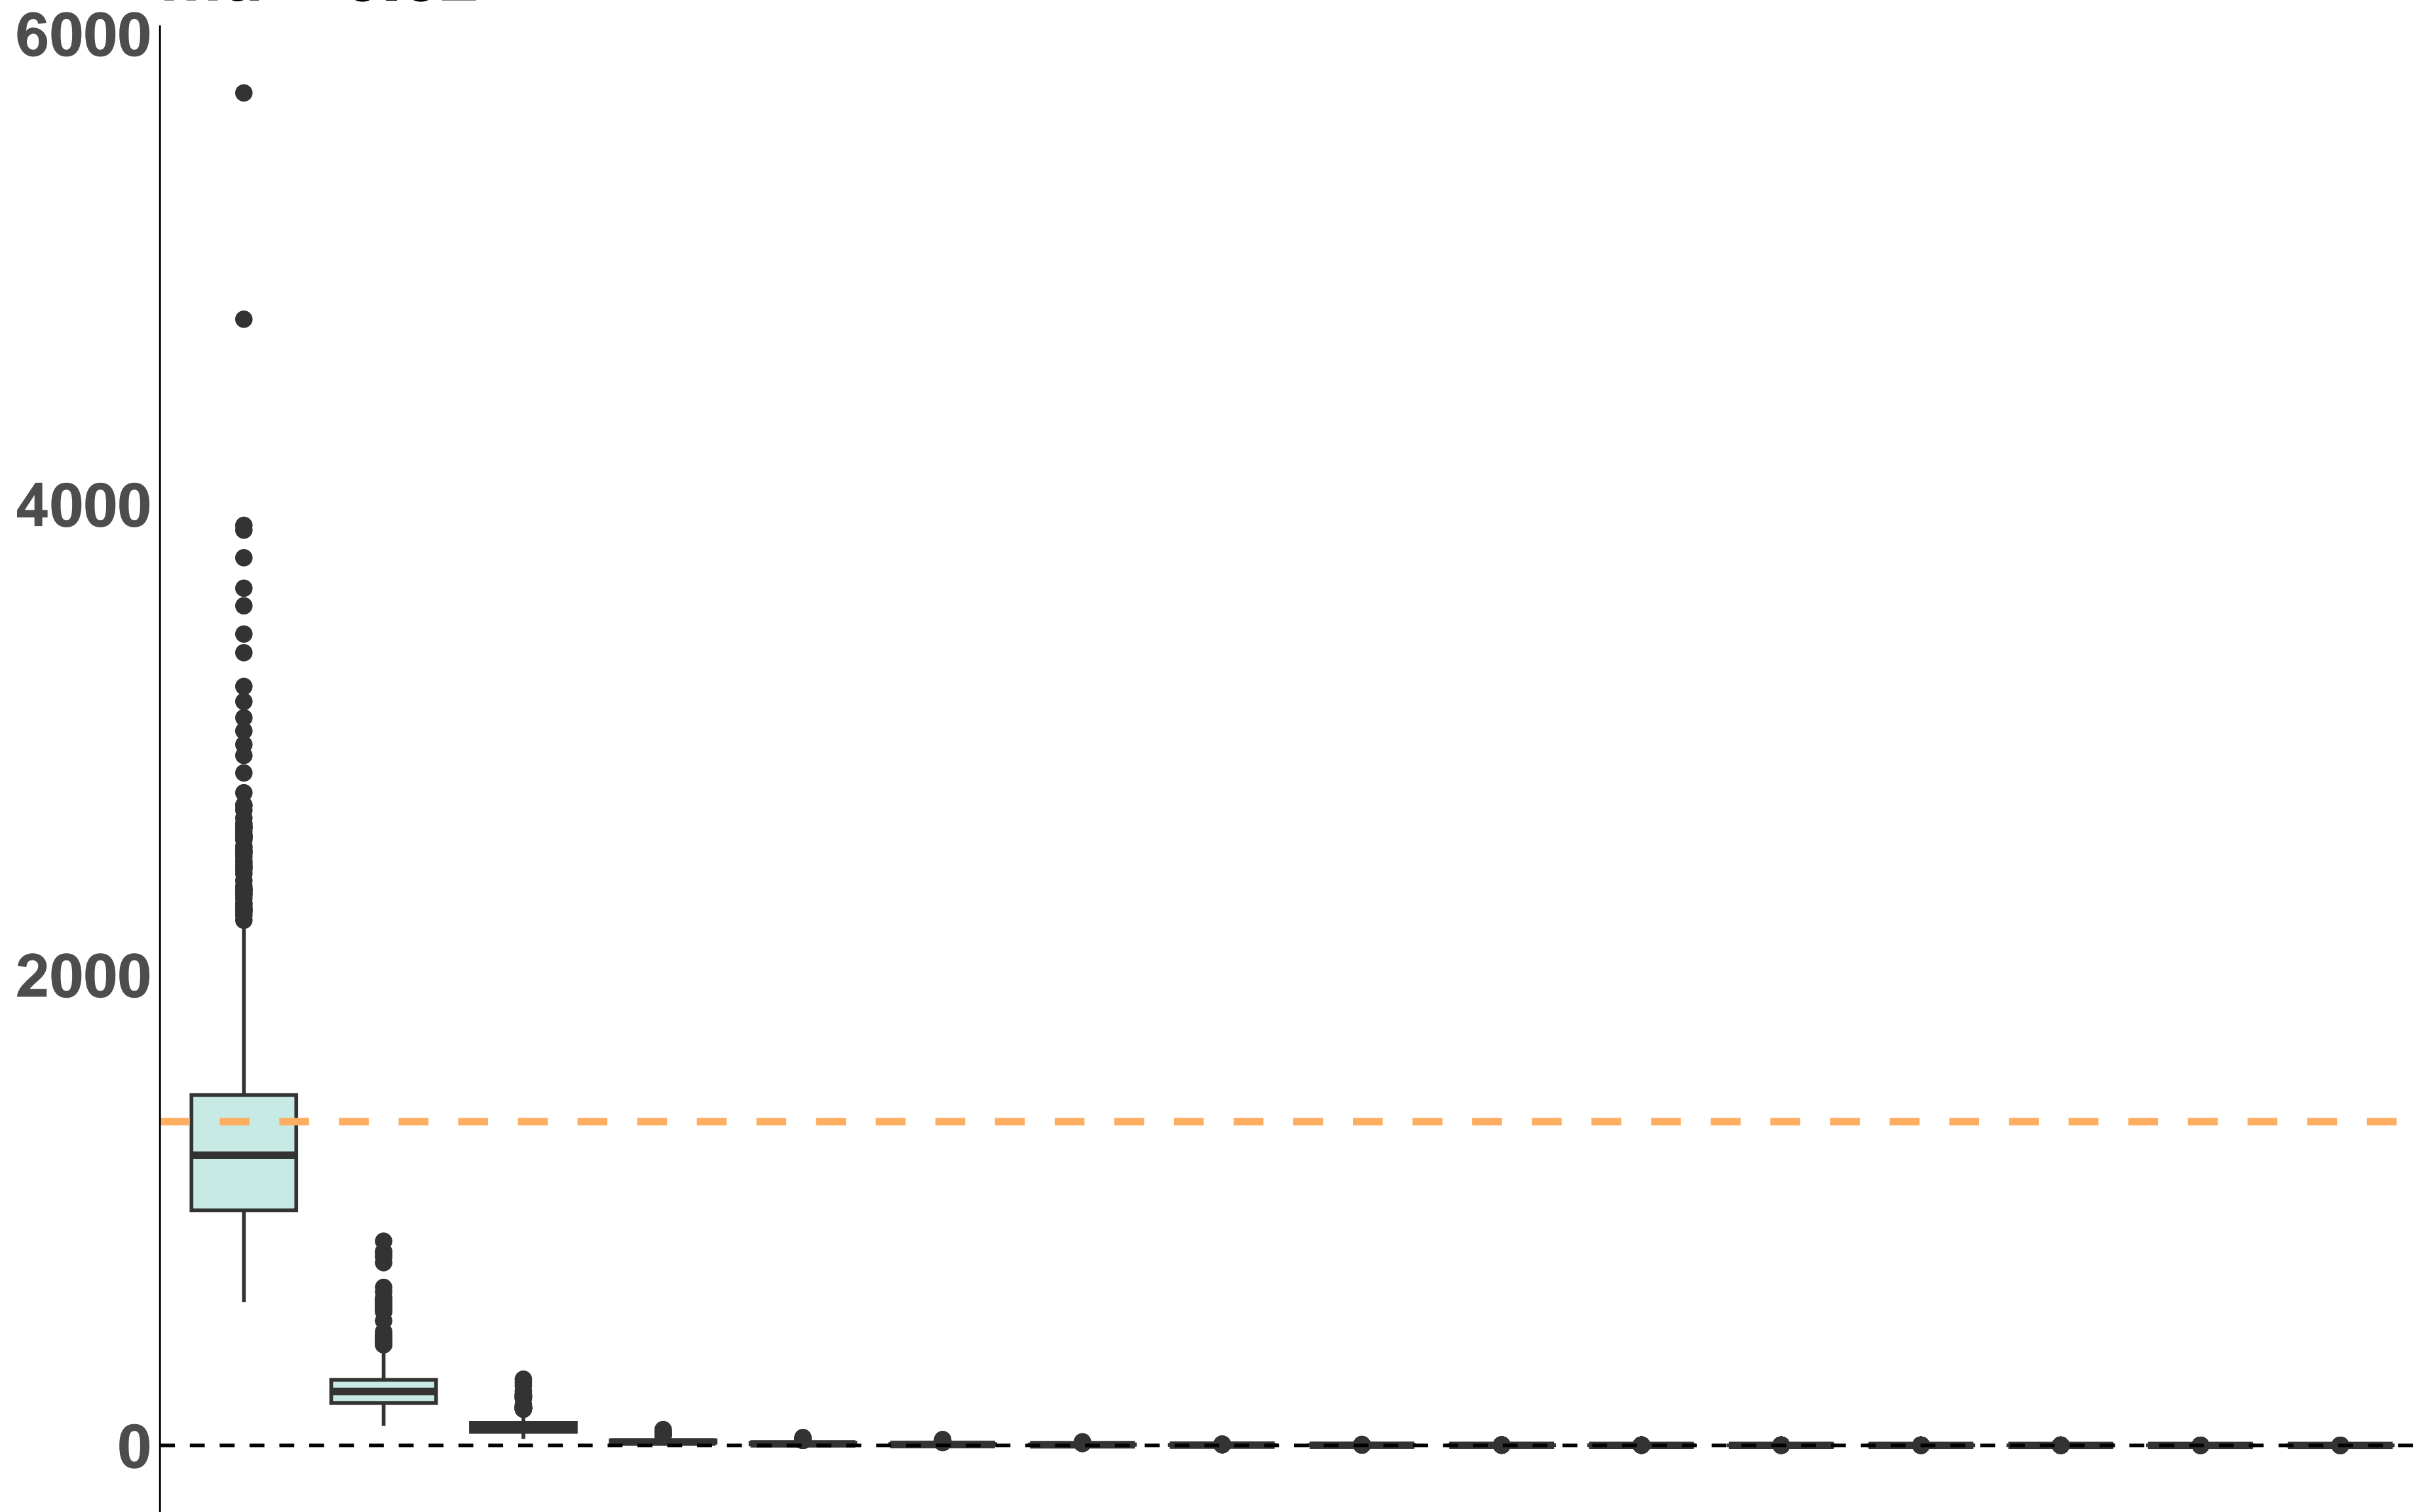

**mu = 0.2**

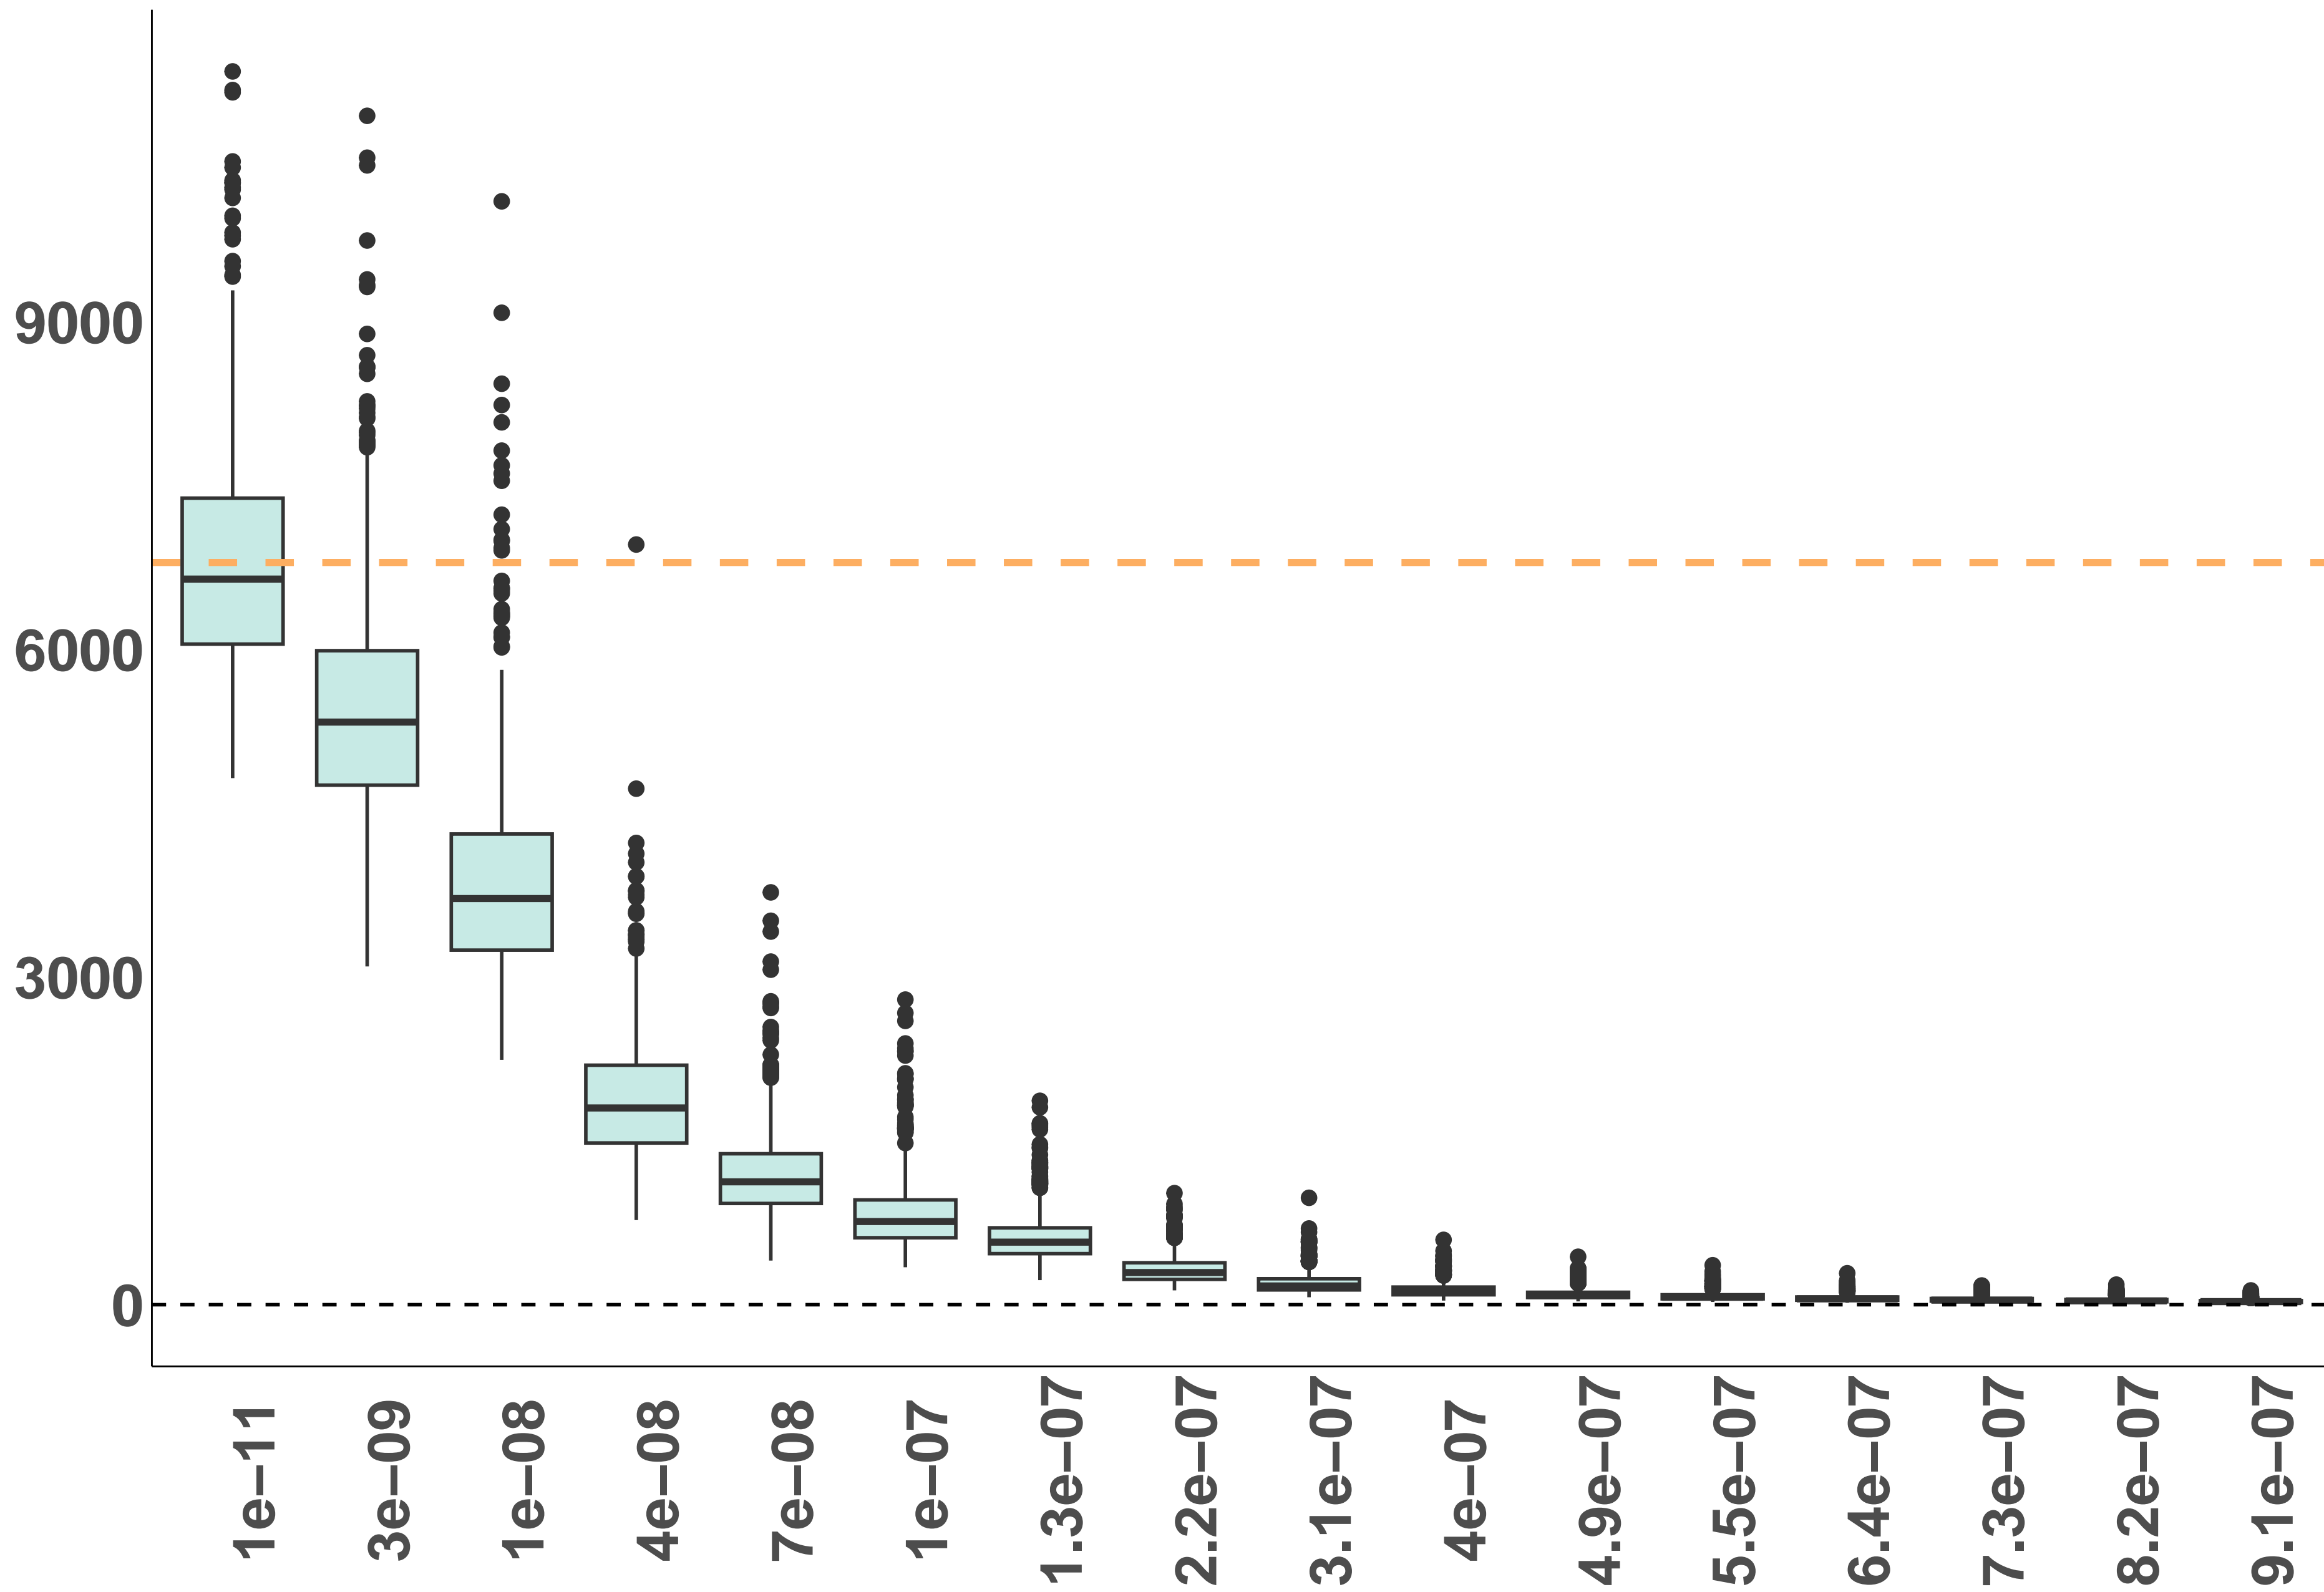

**mu = 0.2**

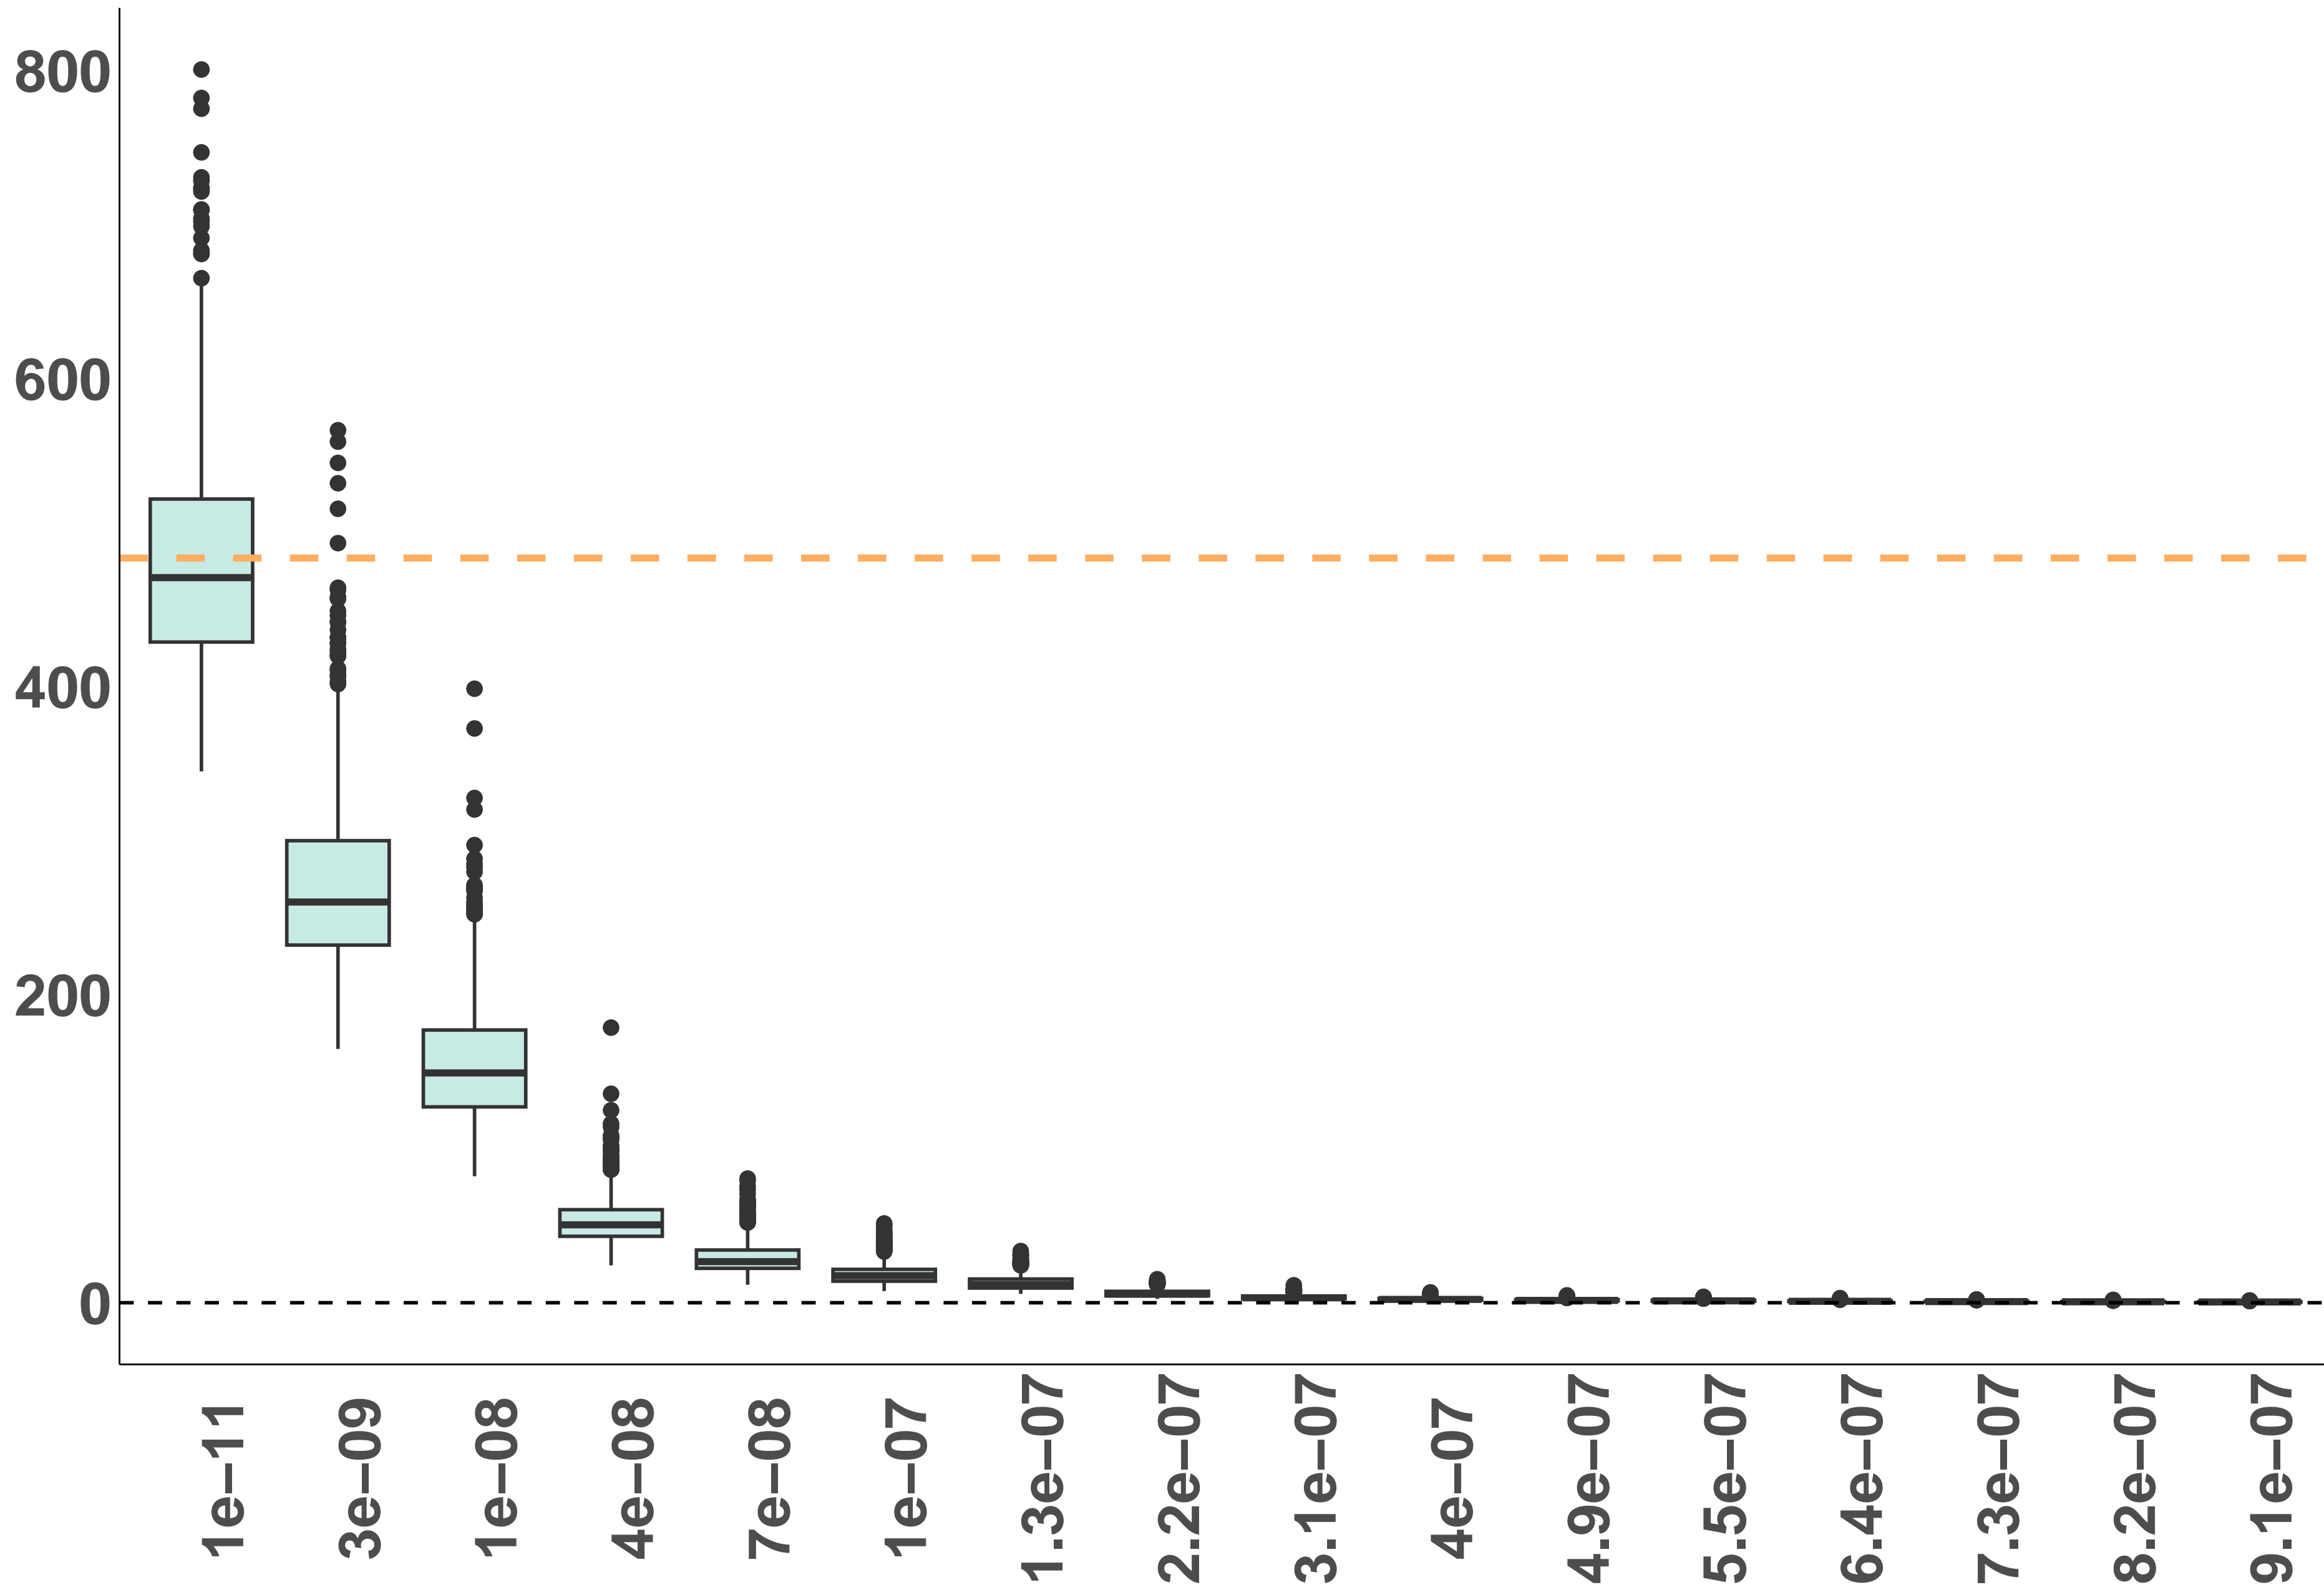

Supplement: Supplementary file 2 [file FigureA2.pdf]
